# Supplementary material for: Random Forest for Dynamic Risk Prediction or Recurrent Events: A Pseudo-Observation Approach
Source: arXiv:2312.00770 source file (2025-02-10)
Supplement: Supplementary file 2 [file Gu_et_al_published_version-_supplementary.pdf]

# Internet Appendix

## A Monte Carlo Simulations

To demonstrate the finite sample performance of all machine learning procedures, we simulate a (latent) 3-factor model for excess returns  $r_{t+1}$ , for  $t = 1, 2, \dots, T$ :

$$r_{i,t+1} = g^*(z_{i,t}) + e_{i,t+1}, \quad e_{i,t+1} = \beta_{i,t} v_{t+1} + \varepsilon_{i,t+1}, \quad z_{i,t} = (1, x_t)' \otimes c_{i,t}, \quad \beta_{i,t} = (c_{i1,t}, c_{i2,t}, c_{i3,t}),$$

where  $c_t$  is an  $N \times P_c$  matrix of characteristics,  $v_{t+1}$  is a  $3 \times 1$  vector of factors,  $x_t$  is a univariate time series, and  $\varepsilon_{t+1}$  is a  $N \times 1$  vector of idiosyncratic errors. We choose  $v_{t+1} \sim \mathcal{N}(0, 0.05^2 \times \mathbb{I}_3)$ , and  $\varepsilon_{i,t+1} \sim t_5(0, 0.05^2)$ , in which their variances are calibrated so that the average time series  $R^2$  is 40% and the average annualized volatility is 30%.

We simulate the panel of characteristics for each  $1 \leq i \leq N$  and each  $1 \leq j \leq P_c$  from the following model:

$$c_{ij,t} = \frac{2}{N+1} \text{CSrank}(\bar{c}_{ij,t}) - 1, \quad \bar{c}_{ij,t} = \rho_j \bar{c}_{ij,t-1} + \epsilon_{ij,t}, \quad (\text{A.1})$$

where  $\rho_j \sim \mathcal{U}[0.9, 1]$ ,  $\epsilon_{ij,t} \sim \mathcal{N}(0, 1 - \rho_j^2)$  and CSrank is Cross-Section rank function, so that the characteristics feature some degree of persistence over time, yet is cross-sectionally normalized to be within  $[-1, 1]$ . This matches our data cleaning procedure in the empirical study.

In addition, we simulate the time series  $x_t$  from the following model:

$$x_t = \rho x_{t-1} + u_t, \quad (\text{A.2})$$

where  $u_t \sim \mathcal{N}(0, 1 - \rho^2)$ , and  $\rho = 0.95$  so that  $x_t$  is highly persistent.

We consider two cases of  $g^*(\cdot)$  functions:

- (a)  $g^*(z_{i,t}) = (c_{i1,t}, c_{i2,t}, c_{i3,t} \times x_t) \theta_0$ , where  $\theta_0 = (0.02, 0.02, 0.02)'$ ;
- (b)  $g^*(z_{i,t}) = (c_{i1,t}^2, c_{i1,t} \times c_{i2,t}, \text{sgn}(c_{i3,t} \times x_t)) \theta_0$ , where  $\theta_0 = (0.04, 0.03, 0.012)'$ .

In both cases,  $g^*(\cdot)$  only depends on 3 covariates, so there are only 3 non-zero entries in  $\theta$ , denoted as  $\theta_0$ . Case (a) is simple and sparse linear model. Case (b) involves a nonlinear covariate  $c_{i1,t}^2$ , a nonlinear and interaction term  $c_{i1,t} \times c_{i2,t}$ , and a discrete variable  $\text{sgn}(c_{i3,t} \times x_t)$ . We calibrate the values of  $\theta_0$  such that the cross-sectional  $R^2$  is 50%, and the predictive  $R^2$  is 5%.

Throughout, we fix  $N = 200$ ,  $T = 180$ , and  $P_x = 2$ , while comparing the cases of  $P_c = 100$  and  $P_c = 50$ , corresponding to  $P = 200$  and 100, respectively, to demonstrate the effect of increasing dimensionality.

For each Monte Carlo sample, we divide the whole time series into 3 consecutive subsamples of equal length for training, validation, and testing, respectively. Specifically, we estimate each of the

Table A.1: Comparison of Predictive  $R^2$ s for Machine Learning Algorithms in Simulations

| Model     | (a)        |      |             |       | (b)        |       |             |       |
|-----------|------------|------|-------------|-------|------------|-------|-------------|-------|
| Parameter | $P_c = 50$ |      | $P_c = 100$ |       | $P_c = 50$ |       | $P_c = 100$ |       |
| $R^2(\%)$ | IS         | OOS  | IS          | OOS   | IS         | OOS   | IS          | OOS   |
| OLS       | 7.50       | 1.14 | 8.19        | -1.35 | 3.44       | -4.72 | 4.39        | -7.75 |
| OLS+H     | 7.48       | 1.25 | 8.16        | -1.15 | 3.43       | -4.60 | 4.36        | -7.54 |
| PCR       | 2.69       | 0.90 | 1.70        | 0.43  | 0.65       | 0.02  | 0.41        | -0.01 |
| PLS       | 6.24       | 3.48 | 6.19        | 2.82  | 1.02       | -0.08 | 0.99        | -0.17 |
| Lasso     | 6.04       | 4.26 | 6.08        | 4.25  | 1.36       | 0.58  | 1.36        | 0.61  |
| Lasso+H   | 6.00       | 4.26 | 6.03        | 4.25  | 1.32       | 0.59  | 1.31        | 0.61  |
| Ridge     | 6.46       | 3.89 | 6.67        | 3.39  | 1.66       | 0.34  | 1.76        | 0.23  |
| Ridge+H   | 6.42       | 3.91 | 6.61        | 3.42  | 1.63       | 0.35  | 1.73        | 0.25  |
| ENet      | 6.04       | 4.26 | 6.08        | 4.25  | 1.35       | 0.58  | 1.35        | 0.61  |
| ENet+H    | 6.00       | 4.26 | 6.03        | 4.25  | 1.32       | 0.59  | 1.31        | 0.61  |
| GLM       | 5.91       | 4.11 | 5.94        | 4.08  | 3.38       | 1.22  | 3.31        | 1.17  |
| GLM+H     | 5.85       | 4.12 | 5.88        | 4.09  | 3.32       | 1.24  | 3.24        | 1.20  |
| RF        | 8.34       | 3.35 | 8.23        | 3.30  | 8.05       | 3.07  | 8.22        | 3.02  |
| GBRT      | 7.08       | 3.35 | 7.02        | 3.33  | 6.51       | 2.76  | 6.42        | 2.84  |
| GBRT+H    | 7.16       | 3.45 | 7.11        | 3.37  | 6.47       | 3.12  | 6.37        | 3.22  |
| NN1       | 6.53       | 4.37 | 6.72        | 4.28  | 5.61       | 2.78  | 5.80        | 2.59  |
| NN2       | 6.55       | 4.42 | 6.72        | 4.26  | 6.22       | 3.13  | 6.33        | 2.91  |
| NN3       | 6.47       | 4.34 | 6.67        | 4.27  | 6.03       | 2.96  | 6.09        | 2.68  |
| NN4       | 6.47       | 4.31 | 6.66        | 4.24  | 5.94       | 2.81  | 6.04        | 2.51  |
| NN5       | 6.41       | 4.27 | 6.55        | 4.14  | 5.81       | 2.72  | 5.70        | 2.20  |
| Oracle    | 6.22       | 5.52 | 6.22        | 5.52  | 5.86       | 5.40  | 5.86        | 5.40  |

Note: In this table, we report the average in-sample (IS) and out-of-sample (OOS)  $R^2$  for models (a) and (b) using Ridge, Lasso, Elastic Net (ENet), generalized linear model with group lasso (GLM), random forest (RF), gradient boosted regression trees (GBRT), and five architectures of neural networks (NN1,...,NN5), respectively. “+H” indicates the use of Huber loss instead of the  $l_2$  loss. “Oracle” stands for using the true covariates in a pooled-OLS regression. We fix  $N = 200$ ,  $T = 180$ , and  $P_x = 2$ , comparing  $P_c = 100$  with  $P_c = 50$ . The number of Monte Carlo repetitions is 100.

two models in the training sample, using PLS, PCR, Ridge, Lasso, Elastic Net (ENet), generalized linear model with group lasso (GLM), random forest (RF), gradient boosted regression trees (GBRT), and the same five architectures of neural networks (NN1,...,NN5) we adopt for the empirical work, respectively, then choose tuning parameters for each method in the validation sample, and calculate the prediction errors in the testing sample. For benchmark, we also compare the pooled OLS with all covariates and that using the oracle model.

We report the average  $R^2$ s both in-sample (IS) and out-of-sample (OOS) for each model and each method over 100 Monte Carlo repetitions in Table A.1. Both IS and OOS  $R^2$  are relative to the estimator based on the IS average. For model (a), Lasso, ENet and NNs deliver the best and almost identical out-of-sample  $R^2$ . This is not surprising given that the true model is sparse and linear in the input covariates. The advanced tree methods such as RF and GBRT tend to overfit, so their performance is slightly worse. By contrast, for model (b), these methods clearly dominate Lasso and ENet, because the latter cannot capture the nonlinearity in the model. GLM is slightly better, but is dominated by NNs, RF, and GBRT. OLS is the worst in all settings, not surprisingly. PLS outperforms PCR in the linear model (a), but is dominated in the nonlinear case. When  $P_c$  increases, the IS  $R^2$  tends to increase whereas the out-of-sample  $R^2$  decreases. Hence,

Table A.2: Comparison of Predictive  $R^2$ s for Alternative Prediction Horizons in Simulations

| Model     | (a)     |       |          |       |        |       | (b)     |        |          |        |        |        |
|-----------|---------|-------|----------|-------|--------|-------|---------|--------|----------|--------|--------|--------|
| Horizon   | Quarter |       | Halfyear |       | Annual |       | Quarter |        | Halfyear |        | Annual |        |
| $R^2$ (%) | IS      | OOS   | IS       | OOS   | IS     | OOS   | IS      | OOS    | IS       | OOS    | IS     | OOS    |
| OLS       | 18.84   | -0.90 | 27.67    | 0.19  | 35.40  | -0.15 | 10.03   | -16.47 | 15.02    | -23.48 | 20.19  | -30.73 |
| OLS+H     | 18.82   | -0.76 | 27.66    | 0.31  | 35.38  | -0.09 | 10.00   | -16.27 | 14.99    | -23.32 | 20.15  | -30.66 |
| PCR       | 3.86    | 0.91  | 5.50     | 1.32  | 7.58   | 1.39  | 0.90    | -0.04  | 1.30     | -0.04  | 1.71   | -0.24  |
| PLS       | 15.12   | 6.56  | 21.52    | 8.40  | 26.46  | 8.14  | 1.91    | -0.42  | 1.73     | -0.33  | 2.78   | -0.80  |
| Lasso     | 14.10   | 10.33 | 20.42    | 14.68 | 25.06  | 16.76 | 3.10    | 1.17   | 4.03     | 1.12   | 4.87   | 0.40   |
| Lasso+H   | 14.01   | 10.32 | 20.30    | 14.67 | 24.85  | 16.74 | 3.03    | 1.19   | 3.91     | 1.15   | 4.66   | 0.48   |
| Ridge     | 15.76   | 7.81  | 23.26    | 10.67 | 29.27  | 11.65 | 4.07    | 0.43   | 5.66     | 0.44   | 6.72   | 0.00   |
| Ridge+H   | 15.68   | 7.84  | 23.15    | 10.69 | 29.13  | 11.65 | 4.00    | 0.45   | 5.56     | 0.46   | 6.56   | 0.04   |
| ENet      | 14.08   | 10.33 | 20.49    | 14.69 | 25.06  | 16.69 | 3.10    | 1.15   | 4.07     | 1.14   | 4.80   | 0.41   |
| ENet+H    | 13.99   | 10.32 | 20.37    | 14.68 | 24.85  | 16.67 | 3.02    | 1.17   | 3.95     | 1.18   | 4.60   | 0.48   |
| GLM       | 13.90   | 9.40  | 21.02    | 13.53 | 27.15  | 15.36 | 7.61    | 2.46   | 10.79    | 2.88   | 13.07  | 1.63   |
| GLM+H     | 13.79   | 9.42  | 20.88    | 13.56 | 26.99  | 15.40 | 7.48    | 2.51   | 10.59    | 2.93   | 12.77  | 1.71   |
| RF        | 17.56   | 8.11  | 25.24    | 11.86 | 31.04  | 14.32 | 15.52   | 5.91   | 20.53    | 7.11   | 22.48  | 6.05   |
| GBRT      | 15.98   | 8.94  | 22.68    | 13.27 | 28.68  | 15.06 | 12.39   | 5.87   | 15.85    | 6.90   | 18.08  | 5.99   |
| GBRT+H    | 15.70   | 8.78  | 22.84    | 13.45 | 29.07  | 15.29 | 12.12   | 5.87   | 16.00    | 7.13   | 18.20  | 6.17   |
| NN1       | 15.68   | 9.99  | 23.04    | 14.07 | 29.62  | 15.58 | 13.25   | 5.36   | 17.95    | 6.29   | 20.68  | 5.32   |
| NN2       | 15.56   | 9.96  | 22.72    | 14.00 | 28.90  | 16.01 | 13.29   | 5.76   | 17.95    | 6.78   | 20.10  | 5.43   |
| NN3       | 15.45   | 9.98  | 22.66    | 13.94 | 28.59  | 16.10 | 13.11   | 5.57   | 17.50    | 6.63   | 20.31  | 5.27   |
| NN4       | 15.49   | 9.91  | 22.32    | 14.06 | 28.59  | 15.97 | 13.20   | 5.56   | 17.90    | 6.52   | 19.67  | 5.20   |
| NN5       | 15.19   | 9.82  | 22.14    | 13.85 | 28.22  | 15.92 | 13.00   | 5.24   | 17.15    | 6.19   | 18.86  | 5.08   |
| Oracle    | 14.37   | 12.72 | 20.73    | 18.15 | 25.42  | 21.56 | 10.91   | 10.28  | 13.61    | 12.75  | 13.04  | 11.52  |

Note: In this table, we report the average in-sample (IS) and out-of-sample (OOS)  $R^2$ s for models (a) and (b) using Ridge, Lasso, Elastic Net (ENet), generalized linear model with group lasso (GLM), random forest (RF), gradient boosted regression trees (GBRT), and five architectures of neural networks (NN1,...,NN5), respectively. “+H” indicates the use of Huber loss instead of the  $l_2$  loss. “Oracle” stands for using the true covariates in a pooled-OLS regression. We fix  $N = 200$ ,  $T = 180$ ,  $P_x = 2$  and  $P_c = 100$ , comparing the performance of different horizons. The number of Monte Carlo repetitions is 100.

the performance of all methods deteriorates as overfitting exacerbates. Using Huber loss improves the out-of-sample performance for almost all methods. RF, GBRT plus Huber loss remain the best choices for the nonlinear model. The comparison among NNs demonstrates a stark trade-off between model flexibility and implementation difficulty. Deeper models potentially allow for more parsimonious representation of the data, but their objective functions are more involved to optimize. For instance, the APG algorithm used in Elastic Net is not feasible for NNs, because its loss (as a function of weight parameters) is non-convex. As shown in the table, shallower NNs tend to outperform.

Table A.2 presents the same IS and OOS  $R^2$ s for prediction conducted for different horizons, e.g., quarterly, half-yearly, and annually. We observe the usual increasing/hump-shape patterns of  $R^2$ s against prediction horizons documented in the literature, which is driven by the persistence of covariates. The relative performance across different models maintains the same.

Next, we report the average variable selection frequencies of 6 particular covariates and the average of the remaining  $P - 6$  covariates for models (a) and (b) in Table A.3, using Lasso, Elastic Net, and Group Lasso and their robust versions. We focus on these methods because they all impose

Table A.3: Comparison of Average Variable Selection Frequencies in Simulations

| Model (a)   |         |            |            |            |                       |                       |                       |       |
|-------------|---------|------------|------------|------------|-----------------------|-----------------------|-----------------------|-------|
| Parameter   | Method  | $c_{i1,t}$ | $c_{i2,t}$ | $c_{i3,t}$ | $c_{i1,t} \times x_t$ | $c_{i2,t} \times x_t$ | $c_{i3,t} \times x_t$ | Noise |
| $P_c = 50$  | Lasso   | 0.95       | 0.94       | 0.65       | 0.53                  | 0.51                  | 0.85                  | 0.09  |
|             | Lasso+H | 0.95       | 0.94       | 0.63       | 0.53                  | 0.50                  | 0.86                  | 0.08  |
|             | ENet    | 0.95       | 0.94       | 0.65       | 0.54                  | 0.51                  | 0.86                  | 0.09  |
|             | ENet+H  | 0.95       | 0.94       | 0.64       | 0.53                  | 0.50                  | 0.86                  | 0.09  |
|             | GLM     | 0.95       | 0.95       | 0.72       | 0.61                  | 0.63                  | 0.90                  | 0.13  |
|             | GLM+H   | 0.95       | 0.94       | 0.70       | 0.61                  | 0.62                  | 0.90                  | 0.12  |
| $P_c = 100$ | Lasso   | 0.95       | 0.94       | 0.65       | 0.52                  | 0.49                  | 0.85                  | 0.06  |
|             | Lasso+H | 0.95       | 0.94       | 0.63       | 0.53                  | 0.49                  | 0.86                  | 0.06  |
|             | ENet    | 0.95       | 0.94       | 0.65       | 0.53                  | 0.49                  | 0.86                  | 0.06  |
|             | ENet+H  | 0.95       | 0.94       | 0.64       | 0.53                  | 0.49                  | 0.86                  | 0.06  |
|             | GLM     | 0.95       | 0.94       | 0.72       | 0.58                  | 0.61                  | 0.90                  | 0.09  |
|             | GLM+H   | 0.95       | 0.94       | 0.69       | 0.55                  | 0.60                  | 0.90                  | 0.09  |

  

| Model (b)   |         |            |            |            |                       |                       |                       |       |
|-------------|---------|------------|------------|------------|-----------------------|-----------------------|-----------------------|-------|
| Parameter   | Method  | $c_{i1,t}$ | $c_{i2,t}$ | $c_{i3,t}$ | $c_{i1,t} \times x_t$ | $c_{i2,t} \times x_t$ | $c_{i3,t} \times x_t$ | Noise |
| $P_c = 50$  | Lasso   | 0.26       | 0.26       | 0.39       | 0.27                  | 0.31                  | 0.75                  | 0.04  |
|             | Lasso+H | 0.25       | 0.25       | 0.38       | 0.28                  | 0.31                  | 0.75                  | 0.04  |
|             | ENet    | 0.26       | 0.25       | 0.39       | 0.27                  | 0.31                  | 0.76                  | 0.04  |
|             | ENet+H  | 0.25       | 0.24       | 0.39       | 0.28                  | 0.31                  | 0.75                  | 0.04  |
|             | GLM     | 0.80       | 0.54       | 0.68       | 0.68                  | 0.64                  | 0.82                  | 0.21  |
|             | GLM+H   | 0.79       | 0.54       | 0.70       | 0.68                  | 0.62                  | 0.82                  | 0.20  |
| $P_c = 100$ | Lasso   | 0.25       | 0.25       | 0.37       | 0.25                  | 0.31                  | 0.75                  | 0.02  |
|             | Lasso+H | 0.24       | 0.24       | 0.36       | 0.26                  | 0.31                  | 0.75                  | 0.02  |
|             | ENet    | 0.25       | 0.25       | 0.37       | 0.25                  | 0.31                  | 0.76                  | 0.02  |
|             | ENet+H  | 0.24       | 0.24       | 0.37       | 0.26                  | 0.31                  | 0.75                  | 0.02  |
|             | GLM     | 0.80       | 0.52       | 0.67       | 0.65                  | 0.57                  | 0.81                  | 0.14  |
|             | GLM+H   | 0.79       | 0.48       | 0.67       | 0.66                  | 0.56                  | 0.81                  | 0.13  |

Note: In this table, we report the average variable selection frequencies of 6 particular covariates for models (a) and (b) (monthly horizon) using Lasso, Elastic Net (ENet), and generalized linear model with group lasso (GLM), respectively. “+H” indicates the use of Huber loss instead of the  $l_2$  loss. Column “Noise” reports the average selection frequency of the remaining  $P - 6$  covariates. We fix  $N = 200$ ,  $T = 180$ , and  $P_x = 2$ , comparing  $P_c = 100$  with  $P_c = 50$ . The number of Monte Carlo repetitions is 100.

the  $l_1$  penalty and hence encourage variable selection. As expected, for model (a), the true covariates ( $c_{i1,t}$ ,  $c_{i2,t}$ ,  $c_{i3,t} \times x_t$ ) are selected in over 85% of the sample paths, whereas correlated yet redundant covariates ( $c_{i3,t}$ ,  $c_{i1,t} \times x_t$ ,  $c_{i2,t} \times x_t$ ) are also selected in around 60% of the samples. By contrast, the remaining covariates are rarely selected. Although model selection mistakes are unavoidable, perhaps due to the tension between variable selection and prediction or for finite sample issues, the true covariates are part of the selected models with high probabilities. For model (b), while no covariates are part of the true model, the 6 covariates we present are more relevant, and hence selected substantially more frequently than the remaining  $P - 6$  ones.

Finally, we report the average VIPs of the 6 particular covariates and the average of the remaining  $P - 6$  covariates for models (a) and (b) in Table A.4, using random forest (RF) and gradient boosted regression trees (GBRT), along with neural networks. We find similar results for both models (a)

Table A.4: Comparison of Average Variable Importance in Simulations

| Model (a)   |        |            |            |            |                       |                       |                       |       |
|-------------|--------|------------|------------|------------|-----------------------|-----------------------|-----------------------|-------|
| Parameter   | Method | $c_{i1,t}$ | $c_{i2,t}$ | $c_{i3,t}$ | $c_{i1,t} \times x_t$ | $c_{i2,t} \times x_t$ | $c_{i3,t} \times x_t$ | Noise |
| $P_c = 50$  | RF     | 21.54      | 23.20      | 5.89       | 6.44                  | 6.42                  | 19.45                 | 0.18  |
|             | GBRT   | 23.86      | 27.86      | 5.64       | 6.41                  | 6.03                  | 25.66                 | 0.05  |
|             | GBRT+H | 24.01      | 27.43      | 5.33       | 6.30                  | 6.78                  | 25.88                 | 0.05  |
|             | NN1    | 26.50      | 29.55      | 5.31       | 2.99                  | 3.75                  | 25.18                 | 0.07  |
|             | NN2    | 26.35      | 28.93      | 5.04       | 3.12                  | 3.93                  | 25.74                 | 0.07  |
|             | NN3    | 26.05      | 28.61      | 5.03       | 3.09                  | 3.89                  | 25.57                 | 0.08  |
|             | NN4    | 26.09      | 28.72      | 5.08       | 3.37                  | 3.82                  | 25.59                 | 0.08  |
|             | NN5    | 25.95      | 28.40      | 5.12       | 3.31                  | 3.73                  | 25.36                 | 0.09  |
| $P_c = 100$ | RF     | 21.40      | 23.08      | 5.84       | 5.62                  | 5.87                  | 19.18                 | 0.10  |
|             | GBRT   | 23.87      | 27.82      | 5.32       | 6.20                  | 5.87                  | 25.43                 | 0.03  |
|             | GBRT+H | 23.75      | 27.12      | 5.20       | 6.04                  | 6.30                  | 26.00                 | 0.03  |
|             | NN1    | 25.78      | 28.36      | 5.03       | 2.77                  | 3.60                  | 24.57                 | 0.05  |
|             | NN2    | 25.30      | 27.88      | 4.85       | 2.95                  | 3.52                  | 24.58                 | 0.06  |
|             | NN3    | 25.32      | 28.03      | 4.73       | 2.89                  | 3.50                  | 24.53                 | 0.06  |
|             | NN4    | 25.02      | 27.63      | 4.77       | 2.92                  | 3.49                  | 24.34                 | 0.06  |
|             | NN5    | 24.78      | 27.73      | 4.82       | 3.07                  | 3.54                  | 24.19                 | 0.06  |
| Model (b)   |        |            |            |            |                       |                       |                       |       |
| Parameter   | Method | $c_{i1,t}$ | $c_{i2,t}$ | $c_{i3,t}$ | $c_{i1,t} \times x_t$ | $c_{i2,t} \times x_t$ | $c_{i3,t} \times x_t$ | Noise |
| $P_c = 50$  | RF     | 27.70      | 6.47       | 5.03       | 8.02                  | 5.00                  | 32.13                 | 0.17  |
|             | GBRT   | 31.24      | 7.37       | 5.82       | 8.81                  | 6.43                  | 36.41                 | 0.04  |
|             | GBRT+H | 32.05      | 7.46       | 5.83       | 8.87                  | 6.62                  | 35.57                 | 0.04  |
|             | NN1    | 55.55      | 14.50      | 4.53       | 3.46                  | 2.97                  | 12.11                 | 0.07  |
|             | NN2    | 51.84      | 13.66      | 4.15       | 2.96                  | 2.72                  | 18.32                 | 0.07  |
|             | NN3    | 52.00      | 13.64      | 4.36       | 2.93                  | 2.89                  | 16.63                 | 0.08  |
|             | NN4    | 51.07      | 13.61      | 4.45       | 3.31                  | 2.81                  | 16.19                 | 0.09  |
|             | NN5    | 49.74      | 13.68      | 4.48       | 3.28                  | 2.86                  | 15.91                 | 0.11  |
| $P_c = 100$ | RF     | 26.42      | 5.74       | 4.40       | 7.77                  | 4.69                  | 31.93                 | 0.10  |
|             | GBRT   | 31.49      | 7.30       | 5.38       | 8.61                  | 6.17                  | 36.70                 | 0.02  |
|             | GBRT+H | 32.13      | 7.48       | 5.71       | 8.66                  | 6.30                  | 35.87                 | 0.02  |
|             | NN1    | 53.09      | 13.53      | 4.79       | 3.45                  | 2.77                  | 12.11                 | 0.05  |
|             | NN2    | 50.25      | 12.93      | 4.26       | 2.87                  | 2.45                  | 17.31                 | 0.05  |
|             | NN3    | 50.36      | 13.00      | 4.30       | 2.90                  | 2.54                  | 15.43                 | 0.06  |
|             | NN4    | 48.28      | 13.05      | 4.50       | 3.21                  | 2.63                  | 15.05                 | 0.07  |
|             | NN5    | 43.44      | 12.41      | 4.71       | 3.61                  | 2.59                  | 16.09                 | 0.09  |

Note: In this table, we report the average variable importance of 6 particular covariates for models (a) and (b) (monthly horizon) using random forest (RF), gradient boosted regression trees (GBRT), and five architectures of neural networks (NN1,...,NN5), respectively. “+H” indicates the use of Huber loss instead of the  $l_2$  loss. Column “Noise” reports the average variable importance of the remaining  $P - 6$  covariates. We fix  $N = 200$ ,  $T = 180$ , and  $P_x = 2$ , comparing  $P_c = 100$  with  $P_c = 50$ . The number of Monte Carlo repetitions is 100.

and (b) that the 6 covariates we present are substantially more important than the remaining  $P - 6$  ones. All methods work equally well.

Overall, the simulation results suggest that the machine learning methods are successful in singling out informative variables, even though highly correlated covariates are difficult to distinguish. This is not surprising, as these methods are implemented to improve prediction, for which purpose

the best model often does not agree with the true model, in particular when covariates are highly correlated.

## B Algorithms in Details

### B.1 Lasso, Ridge, Elastic Net, and Group Lasso

We present the accelerated proximal algorithm (APG), see, e.g., [Parikh and Boyd \(2013\)](#) and [Polson et al. \(2015\)](#)., which allows for efficient implementation of the elastic net, Lasso, Ridge regression, and Group Lasso for both  $l_2$  and Huber losses. We rewrite their regularized objective functions as

$$\mathcal{L}(\theta; \cdot) = \underbrace{\mathcal{L}(\theta)}_{\text{Loss Function}} + \underbrace{\phi(\theta; \cdot)}_{\text{Penalty}}, \quad (\text{B.3})$$

where we omit the dependence on the tuning parameters. Specifically, we have

$$\phi(\theta; \cdot) = \begin{cases} \frac{1}{2}\lambda \sum_{j=1}^P \theta_j^2, & \text{Ridge;} \\ \lambda \sum_{j=1}^P |\theta_j|, & \text{Lasso;} \\ \lambda(1-\rho) \sum_{j=1}^P |\theta_j| + \frac{1}{2}\lambda\rho \sum_{j=1}^P \theta_j^2, & \text{Elastic Net;} \\ \lambda \sum_{j=1}^P \|\theta_j\|, & \text{Group Lasso.} \end{cases}, \quad (\text{B.4})$$

where in the Group Lasso case,  $\theta = (\theta_1, \theta_2, \dots, \theta_P)$  is a  $K \times P$  matrix.

Proximal algorithms are a class of algorithms for solving convex optimization problems, in which the base operation is evaluating the proximal operator of a function, ie., solving a small convex optimization problem. In many cases, this smaller problem has a closed form solution. The proximal operator is defined as:

$$\mathbf{prox}_{\gamma f}(\theta) = \underset{z}{\operatorname{argmin}} \left\{ f(z) + \frac{1}{2\gamma} \|z - \theta\|^2 \right\}.$$

An important property of the proximal operator is that the minimizer of a convex function  $f(\cdot)$  is a fixed point of  $\mathbf{prox}_f(\cdot)$ , i.e.,  $\theta^*$  minimizes  $f(\cdot)$  if and only if

$$\theta^* = \mathbf{prox}_f(\theta^*).$$

The proximal gradient algorithm is designed to minimize an objective function of the form (B.3), where  $\mathcal{L}(\theta)$  is differentiable function of  $\theta$  but  $\phi(\theta; \cdot)$  is not. Using properties of the proximal operator,

one can show that  $\theta^*$  minimizes (B.3), if and only if

$$\theta^* = \mathbf{prox}_{\gamma\phi}(\theta^* - \gamma\nabla\mathcal{L}(\theta^*)).$$

This result motivates the first two iteration steps in Algorithm 1. The third step inside the while loop is a Nesterov momentum (Nesterov (1983)) adjustment that accelerates convergence.

The optimization problem requires the proximal operators of  $\phi(\theta; \cdot)$ s in (B.4), which have closed forms:

$$\mathbf{prox}_{\gamma\phi}(\theta) = \begin{cases} \frac{\theta}{1 + \lambda\gamma}, & \text{Ridge;} \\ \lambda S(\theta, \lambda\gamma), & \text{Lasso;} \\ \frac{1}{1 + \lambda\gamma\rho} S(\theta, (1 - \rho)\lambda\gamma), & \text{Elastic Net;} \\ (\tilde{S}(\theta_1, \lambda\gamma)^\top, \tilde{S}(\theta_2, \lambda\gamma)^\top, \dots, \tilde{S}(\theta_P, \lambda\gamma)^\top)^\top, & \text{Group Lasso.} \end{cases},$$

where  $S(x, \mu)$  and  $\tilde{S}(x, \mu)$  are vector-valued functions, whose  $i$ th components are defined by:

$$(S(x, \mu))_i = \begin{cases} x_i - \mu, & \text{if } x_i > 0 \text{ and } \mu < |x_i|; \\ x_i + \mu, & \text{if } x_i < 0 \text{ and } \mu < |x_i|; \\ 0, & \text{if } \mu \geq |x_i|. \end{cases}, \quad (\tilde{S}(x, \mu))_i = \begin{cases} x_i - \mu \frac{x_i}{\|x_i\|}, & \text{if } \|x_i\| > \mu; \\ 0, & \text{if } \|x_i\| \leq \mu. \end{cases}.$$

Note that  $S(x, \mu)$  is the soft-thresholding operator, so the proximal algorithm is equivalent to the coordinate descent algorithm in the case of  $l_2$  loss, see, e.g., Daubechies et al. (2004), Friedman et al. (2007). The proximal framework we adopt here allows efficient implementation of Huber loss and convergence acceleration.

---

**Algorithm 1:** Accelerated Proximal Gradient Method

---

Initialization:  $\theta_0 = 0$ ,  $m = 0$ ,  $\gamma$ ;

**while**  $\theta_m$  not converged **do**

$\tilde{\theta} \leftarrow \theta_m - \gamma\nabla\mathcal{L}(\theta) |_{\theta=\theta_m}$ .

$\tilde{\theta} \leftarrow \mathbf{prox}_{\gamma\phi}(\tilde{\theta})$ .

$\theta_{m+1} \leftarrow \tilde{\theta} + \frac{m}{m+3}(\tilde{\theta} - \theta_m)$ .

$m \leftarrow m + 1$ .

**end**

**Result:** The final parameter estimate is  $\theta_m$ .

---

## B.2 Tree, Random Forest, and Gradient Boosted Tree

Algorithm 2 is a greedy algorithm, see, e.g., Breiman et al. (1984), to grow a complete binary regression tree. Next, Algorithm 3 yields the random forest, e.g., Hastie et al. (2009). Finally, Algorithm 4 delivers the gradient boosted tree (Friedman (2001)), for which we follow the version written by Bühlmann and Hothorn (2007).

---

### Algorithm 2: Classification and Regression Tree

---

Initialize the stump.  $C_1(0)$  denotes the range of all covariates,  $C_l(d)$  denote the  $l$ -th node of depth  $d$ .

**for**  $d$  from 1 to  $L$  **do**

**for**  $i$  in  $\{C_l(d-1), l = 1, \dots, 2^{d-1}\}$  **do**  $2^{d-1}$  is the number of partitions at the  $d$ -1-th depth

        i) For each feature  $j = 1, 2, \dots, P$ , and each threshold level  $\alpha$ , define a split as  $s = (j, \alpha)$ , which divides  $C_l(d-1)$  into  $C_{left}$  and  $C_{right}$ :

$$C_{left}(s) = \{z_j \leq \alpha\} \cap C_l(d-1); \quad C_{right}(s) = \{z_j > \alpha\} \cap C_l(d-1),$$

        where  $z_j$  denotes the  $j$ th covariate.

        ii) Define the impurity function:

$$\mathcal{L}(C, C_{left}, C_{right}) = \frac{|C_{left}|}{|C|} H(C_{left}) + \frac{|C_{right}|}{|C|} H(C_{right}), \text{ where}$$

$$H(C) = \frac{1}{|C|} \sum_{z_{i,t} \in C} (r_{i,t+1} - \theta)^2, \quad \theta = \frac{1}{|C|} \sum_{z_{i,t} \in C} r_{i,t+1},$$

        and  $|C|$  denotes the number of observations in set  $C$ .

        iii) Select the optimal split:

$$s^* \leftarrow \underset{s}{\operatorname{argmin}} \mathcal{L}(C(s), C_{left}(s), C_{right}(s)).$$

        iv) Update the nodes:

$$C_{2l-1}(d) \leftarrow C_{left}(s^*), \quad C_{2l}(d) \leftarrow C_{right}(s^*).$$

**end**

**end**

**Result:** The output of a regression tree is given by:

$$g(z_{i,t}; \theta, L) = \sum_{k=1}^{2^L} \theta_k \mathbf{1}\{z_{i,t} \in C_k(L)\}, \text{ where } \theta_k = \frac{1}{|C_k(L)|} \sum_{z_{i,t} \in C_k(L)} r_{i,t+1}.$$

For a single binary complete regression tree  $\mathcal{T}$  of depth  $L$ , the VIP for the covariate  $z_j$  is

$$\text{VIP}(z_j, \mathcal{T}) = \sum_{d=1}^{L-1} \sum_{i=1}^{2^{d-1}} \Delta \text{im}(C_i(d-1), C_{2i-1}(d), C_{2i}(d)) \mathbf{1}\{z_j \in \mathcal{T}(i, d)\},$$

where  $\mathcal{T}(i, d)$  represents the covariate on the  $i$ -th (internal) node of depth  $d$ , which splits  $C_i(d-1)$  into two sub-regions  $\{C_{2i-1}(d), C_{2i}(d)\}$ , and  $\Delta \text{im}(\cdot, \cdot, \cdot)$  is defined by:

$$\Delta \text{im}(C, C_{left}, C_{right}) = H(C) - \mathcal{L}(C, C_{left}, C_{right}).$$

not splitting vs splitting given a tree.  
but does it depends on  $z_j$ ?

Yes, only for nodes where the covariate was used for splitting.

---

**Algorithm 3:** Random Forest

---

**for**  $b$  from 1 to  $B$  **do**

Generate Bootstrap samples  $\{(z_{i,t}, r_{i,t+1}), (i, t) \in \text{Bootstrap}(b)\}$  from the original dataset, for which a tree is grown using Algorithm 2. At each step of splitting, use only a random subsample, say  $\sqrt{P}$  or any specific number, of all features. Write the resulting  $b$ th tree as:

$$\hat{g}_b(z_{i,t}; \hat{\theta}_b, L) = \sum_{k=1}^{2^L} \theta_b^{(k)} \mathbf{1}\{z_{i,t} \in C_k(L)\}.$$

**end**

**Result:** The final random forest output is given by the average of the outputs of all  $B$  trees.

$$\hat{g}(z_{i,t}; L, B) = \frac{1}{B} \sum_{b=1}^B \hat{g}_b(z_{i,t}; \hat{\theta}_b, L).$$

---

---

**Algorithm 4:** Gradient Boosted Tree

---

Initialize the predictor as  $\hat{g}_0(\cdot) = 0$ ;

**for**  $b$  from 1 to  $B$  **do**

Compute for each  $i = 1, 2, \dots, N$  and  $t = 1, 2, \dots, T$ , the negative gradient of the loss function  $l(\cdot, \cdot)$ :<sup>a</sup>

$$\varepsilon_{i,t+1} \leftarrow -\frac{\partial l(r_{i,t+1}, g)}{\partial g} \Big|_{g=\hat{g}_{b-1}(z_{i,t})}.$$

this is the gradient.  $l$  is the loss function  
 $g$  is the function approximated by a tree.  
why is this called "residual"?

Grow a (shallow) regression tree of depth  $L$  with dataset  $\{(z_{i,t}, \varepsilon_{i,t+1}) : \forall i, \forall t\}$

$$\hat{f}_b(\cdot) \leftarrow g(z_{i,t}; \theta, L).$$

Update the model by

$$\hat{g}_b(\cdot) \leftarrow \hat{g}_{b-1}(\cdot) + \nu \hat{f}_b(\cdot),$$

where  $\nu \in (0, 1]$  is a tuning parameter that controls the step length.

**end**

**Result:** The final model output is

$$\hat{g}_B(z_{i,t}; B, \nu, L) = \sum_{b=1}^B \nu \hat{f}_b(\cdot).$$

---

<sup>a</sup>The typical choice of  $l(\cdot, \cdot)$  for regression is  $l_2$  or Huber loss, whereas for classification, it is more common to use the following loss function:

$$l(d, g(\cdot)) = \log_2(1 + \exp(-2(2d - 1)g(\cdot))).$$

### B.3 Neural Networks

It is common to fit the neural network using stochastic gradient descent (SGD), see, e.g., Goodfellow et al. (2016). We adopt the **adaptive moment estimation algorithm (Adam)**, an efficient version of the SGD introduced by Kingma and Ba (2014). **Adam computes adaptive learning rates** for individual parameters using estimates of first and second moments of the gradients. We denote the loss function as  $\mathcal{L}(\theta; \cdot)$  and write  $\mathcal{L}(\theta; \cdot) = \frac{1}{T} \sum_{t=1}^T \mathcal{L}_t(\theta; \cdot)$ , where  $\mathcal{L}_t(\theta; \cdot)$  is the penalized cross-sectional average prediction error at time  $t$ . At each step of training, a batch sent to the algorithm is randomly sampled from the training dataset. Algorithm 6 is the early stopping algorithm that can be used in combination with many optimization routines, including Adam. Algorithm 7 gives the Batch-Normalization transform (Ioffe and Szegedy (2015)), which we apply to each activation after ReLU transformation. Any neuron that previously receives a batch of  $x$  as the input now receives  $\text{BN}_{\gamma, \beta}(x)$  instead, where  $\gamma$  and  $\beta$  are additional parameters to be optimized.

---

#### Algorithm 5: Adam for Stochastic Gradient Descent (SGD)

---

Initialize the parameter vector  $\theta_0$ . Set  $m_0 = 0, v_0 = 0, t = 0$ .

**while**  $\theta_t$  not converged **do**

$t \leftarrow t + 1$ .

$g_t \leftarrow \nabla_{\theta} \mathcal{L}_t(\theta; \cdot) |_{\theta=\theta_{t-1}}$ .

$m_t \leftarrow \beta_1 m_{t-1} + (1 - \beta_1) g_t$ .

$v_t \leftarrow \beta_2 v_{t-1} + (1 - \beta_2) g_t \odot g_t$ .<sup>a</sup>

$\hat{m}_t \leftarrow m_t / (1 - (\beta_1)^t)$ .

$\hat{v}_t \leftarrow v_t / (1 - (\beta_2)^t)$ .

$\theta_t \leftarrow \theta_{t-1} - \alpha \hat{m}_t \oslash (\sqrt{\hat{v}_t} + \epsilon)$ .

**end**

**Result:** The final parameter estimate is  $\theta_t$ .

---

<sup>a</sup> $\odot$  and  $\oslash$  denote element-wise multiplication and division, respectively.

---

#### Algorithm 6: Early Stopping

---

Initialize  $j = 0, \epsilon = \infty$  and select the patience parameter  $p$ .

**while**  $j < p$  **do**

Update  $\theta$  using the training algorithm (e.g., the steps inside the while loop of Algorithm 5 for  $h$  steps).

Calculate the prediction error from the validation sample, denoted as  $\epsilon'$ .

**if**  $\epsilon' < \epsilon$  **then**

$j \leftarrow 0$ .

$\epsilon \leftarrow \epsilon'$ .

$\theta' \leftarrow \theta$ .

**else**

$j \leftarrow j + 1$ .

**end**

**end**

**Result:** The final parameter estimate is  $\theta'$ .

---

---

**Algorithm 7:** Batch Normalization (for one Activation over one Batch)

---

Input: Values of  $x$  for each activation over a batch  $\mathcal{B} = \{x_1, x_2, \dots, x_N\}$ .

$$\mu_{\mathcal{B}} \leftarrow \frac{1}{N} \sum_{i=1}^N x_i$$

$$\sigma_{\mathcal{B}}^2 \leftarrow \frac{1}{N} \sum_{i=1}^N (x_i - \mu_{\mathcal{B}})^2$$

$$\hat{x}_i \leftarrow \frac{x_i - \mu_{\mathcal{B}}}{\sqrt{\sigma_{\mathcal{B}}^2 + \epsilon}}$$

$$y_i \leftarrow \gamma \hat{x}_i + \beta := \text{BN}_{\gamma, \beta}(x_i)$$

**Result:**  $\{y_i = \text{BN}_{\gamma, \beta}(x_i) : i = 1, 2, \dots, N\}$ .

---

[lots of useful references.](#)

## C Theoretical Properties of Machine Learning Models

In this section, we provide references on the asymptotic properties of machine learning methods discussed in the main text. The references below are unavoidably selective and by no means complete. We invite interested readers to consult references within the following papers.

For theoretical properties of lasso, see [Knight and Fu \(2000\)](#), [Bickel et al. \(2009\)](#), [Meinshausen and Yu \(2009\)](#), [Tibshirani \(2011\)](#), [Wainwright \(2009\)](#), and [Zhang and Huang \(2008\)](#). And for elastic net, see [Zou and Hastie \(2005\)](#), [Zou and Zhang \(2009\)](#), and [Mol et al. \(2009\)](#). For group Lasso in linear models, see [Lounici et al. \(2011\)](#), and see [Bach \(2008\)](#) and [Ravikumar et al. \(2009\)](#) for additive and nonparametric models. While most theoretical analysis in high-dimensional statistics assume that data have sub-Gaussian or sub-exponential tails, [Fan et al. \(2017\)](#) provide a theoretical justification of using Huber’s loss function in the high-dimensional setting.

For dimension reduction techniques, there is a large literature in statistics on the asymptotic behavior of PCA, e.g., [Bai \(1999\)](#), [Johnstone \(2001\)](#), [Johnstone and Lu \(2009\)](#), [Paul \(2007\)](#), [Wang and Fan \(2017\)](#), and another large literature in econometrics focusing on the asymptotic theory of PCA in modern factor analysis, e.g., [Stock and Watson \(2002\)](#), [Bai and Ng \(2002\)](#), and [Bai and Ng \(2013\)](#). There are, however, fewer results on the asymptotic analysis of PCR and PLS in particular. One can refer to [Giglio and Xiu \(2016\)](#) for the asymptotic theory of PCR in the context of risk premia estimation, and [Kelly and Pruitt \(2013, 2015\)](#) for the theory of PLS with its application to forecasting risk premia in financial markets.

A recent literature analyzes theoretical properties of random forests, see [Biau \(2012\)](#), [Scornet et al. \(2015\)](#), [Mentch and Hooker \(2016\)](#), [Wager et al. \(2014\)](#), and [Wager and Athey \(2018\)](#). The properties of gradient boosting, on the other hand, are well understood from the early work of e.g., [Friedman et al. \(2000\)](#), [Bühlmann and Yu \(2003\)](#), [Lugosi and Vayatis \(2004\)](#), and [Zhang and Yu \(2005\)](#) for both classification and regression problems. However, much work remains to be done to fully take into account optimization and regularization algorithms that are essential to the desirable performance of various boosting methods, e.g., the popular XGBoost system designed by [Chen and Guestrin \(2016\)](#).

Likewise, theoretical properties of neural networks and deep learning are in large part under-developed (for an overview, see [Fan et al., 2019](#)). First, the approximation theory of neural networks

is far from complete. Although earlier work have established a universal approximation theory with a single hidden layer network (e.g., [Hornik et al., 1989](#)), a recent line of work sheds light on the distinction between depth and width of a multi-layer network. [Eldan and Shamir \(2016\)](#) formally demonstrate that depth—even if increased by one layer—can be exponentially more valuable than increasing width in standard feed-forward neural networks (see also [Lin et al., 2017](#); [Rolnick and Tegmark, 2018](#)).

Second, any theoretical understanding of neural networks should explicitly account for the modern optimization algorithms that, in combination with statistical analysis, are critical to their success. But training a deep neural network typically involves a grab bag of algorithms, e.g., SGD, Adam, batch normalization, skipping connections ([He et al., 2016](#)), some of which rely on heuristic explanation without rigorous analysis. A promising recent strand of work [Chizat and Bach \(2018\)](#), [Mei et al. \(2018\)](#), and [Mei et al. \(2019\)](#) approximate the evolution of network weight parameters in the SDG algorithm for networks with a single hidden layer. They show that mean-field partial differential equations accurately describe this process as long as the number of hidden units is sufficiently large. In summary, there remains much work to be done to establish theoretical properties of deep learning.

## D Sample Splitting

We consider a number of sample splitting schemes studied in the forecast evaluation literature (see, e.g., [West, 2006](#)). The “fixed” scheme splits the data into training, validation, and testing samples. It estimates the model once from the training and validation samples, and attempts to fit all points in the testing sample using this fixed model estimate.

A common alternative to the fixed split scheme is a “rolling” scheme, in which the training and validation samples gradually shift forward in time to include more recent data, but holds the total number of time periods in each training and validation sample fixed. For each rolling window, one refits the model from the prevailing training and validation samples, and tracks a model’s performance in the remaining test data that has not been subsumed by the rolling windows. The result is a sequence of performance evaluation measures corresponding to each rolling estimation window. This has the benefit of leveraging more recent information for prediction relative to the fixed scheme.

The third is a “recursive” performance evaluation scheme. Like the rolling approach, it gradually includes more recent observations in the training and validation windows. But the recursive scheme always retains the entire history in the training sample, thus its window size gradually increases. The rolling and recursive schemes are computationally expensive, in particular for more complicated models such as neural networks.

In our empirical exercise, we adopt a hybrid of these schemes by recursively increasing the training sample, periodically refitting the entire model once per year, and making out-of-sample predictions using the same fitted model over the subsequent year. Each time we refit, we increase the training sample by a year, while maintaining a fixed size rolling sample for validation. **We choose to *not* cross-validate in order to maintain the temporal ordering of the data for prediction.**

Table A.5: Hyperparameters For All Methods

|                                      | OLS-3<br>+H | PLS | PCR | ENet<br>+H                                       | GLM<br>+H                                    | RF                                                                                              | GBRT<br>+H                                                                                                                     | NN1 - NN5                                                                                                                                                                                                                                                                                    |
|--------------------------------------|-------------|-----|-----|--------------------------------------------------|----------------------------------------------|-------------------------------------------------------------------------------------------------|--------------------------------------------------------------------------------------------------------------------------------|----------------------------------------------------------------------------------------------------------------------------------------------------------------------------------------------------------------------------------------------------------------------------------------------|
| Huber loss $\xi =$<br>99.9% quantile | ✓           | -   | -   | ✓                                                | ✓                                            | -                                                                                               | ✓                                                                                                                              | -                                                                                                                                                                                                                                                                                            |
| Others                               |             | $K$ | $K$ | $\rho = 0.5$<br>$\lambda \in (10^{-4}, 10^{-1})$ | #Knots=3<br>$\lambda \in (10^{-4}, 10^{-1})$ | Depth= 1 ~ 6<br>#Trees= 300<br>#Features in each split<br>$\in \{3, 5, 10, 20, 30, 50, \dots\}$ | Depth= 1 ~ 2<br>#Trees= 1 ~ 1000<br>Learning Rate<br>LR $\in \{0.01, 0.1\}$<br><br>why did people<br>call it learning<br>rate? | L1 penalty<br>$\lambda_1 \in (10^{-5}, 10^{-3})$ for weights?<br>Learning Rate<br>LR $\in \{0.001, 0.01\}$ ??<br>Batch Size=10000 for SGD<br>Epochs=100<br>Patience=5 for early stopping<br>Adam Para.=Default<br>Ensemble=10 initializations<br><br>each epoch<br>pass through<br>all data. |

Note: The table describes the hyperparameters that we tune in each machine learning method.

## E Hyperparameter Tuning

Table A.5 describes the set of hyperparameters and their potential values used for tuning each machine learning model.

## F Additional Tables and Figures

Table A.6: Details of the Characteristics

| No. | Acronym  | Firm characteristic                        | Paper's author(s)                            | Year, Journal | Data Source    | Frequency |
|-----|----------|--------------------------------------------|----------------------------------------------|---------------|----------------|-----------|
| 1   | absacc   | Absolute accruals                          | Bandyopadhyay, Huang & Wirjanto              | 2010, WP      | Compustat      | Annual    |
| 2   | acc      | Working capital accruals                   | Sloan                                        | 1996, TAR     | Compustat      | Annual    |
| 3   | aeavol   | Abnormal earnings announcement volume      | Lerman, Livnat & Mendenhall                  | 2007, WP      | Compustat+CRSP | Quarterly |
| 4   | age      | # years since first Compustat coverage     | Jiang, Lee & Zhang                           | 2005, RAS     | Compustat      | Annual    |
| 5   | agr      | Asset growth                               | Cooper, Gulen & Schill                       | 2008, JF      | Compustat      | Annual    |
| 6   | baspread | Bid-ask spread                             | Amihud & Mendelson                           | 1989, JF      | CRSP           | Monthly   |
| 7   | beta     | Beta                                       | Fama & MacBeth                               | 1973, JPE     | CRSP           | Monthly   |
| 8   | betasq   | Beta squared                               | Fama & MacBeth                               | 1973, JPE     | CRSP           | Monthly   |
| 9   | bm       | Book-to-market                             | Rosenberg, Reid & Lanstein                   | 1985, JPM     | Compustat+CRSP | Annual    |
| 10  | bm.ia    | Industry-adjusted book to market           | Asness, Porter & Stevens                     | 2000, WP      | Compustat+CRSP | Annual    |
| 11  | cash     | Cash holdings                              | Palazzo                                      | 2012, JFE     | Compustat      | Quarterly |
| 12  | cashdebt | Cash flow to debt                          | Ou & Penman                                  | 1989, JAE     | Compustat      | Annual    |
| 13  | cashpr   | Cash productivity                          | Chandrashekar & Rao                          | 2009, WP      | Compustat      | Annual    |
| 14  | cfp      | Cash flow to price ratio                   | Desai, Rajgopal & Venkatachalam              | 2004, TAR     | Compustat      | Annual    |
| 15  | cfp.ia   | Industry-adjusted cash flow to price ratio | Asness, Porter & Stevens                     | 2000, WP      | Compustat      | Annual    |
| 16  | chatoia  | Industry-adjusted change in asset turnover | Soliman                                      | 2008, TAR     | Compustat      | Annual    |
| 17  | chcsho   | Change in shares outstanding               | Pontiff & Woodgate                           | 2008, JF      | Compustat      | Annual    |
| 18  | chempia  | Industry-adjusted change in employees      | Asness, Porter & Stevens                     | 1994, WP      | Compustat      | Annual    |
| 19  | chiniv   | Change in inventory                        | Thomas & Zhang                               | 2002, RAS     | Compustat      | Annual    |
| 20  | chmom    | Change in 6-month momentum                 | Gettleman & Marks                            | 2006, WP      | CRSP           | Monthly   |
| 21  | chpmia   | Industry-adjusted change in profit margin  | Soliman                                      | 2008, TAR     | Compustat      | Annual    |
| 22  | chtx     | Change in tax expense                      | Thomas & Zhang                               | 2011, JAR     | Compustat      | Quarterly |
| 23  | cinvest  | Corporate investment                       | Titman, Wei & Xie                            | 2004, JFQA    | Compustat      | Quarterly |
| 24  | convind  | Convertible debt indicator                 | Valta                                        | 2016, JFQA    | Compustat      | Annual    |
| 25  | currat   | Current ratio                              | Ou & Penman                                  | 1989, JAE     | Compustat      | Annual    |
| 26  | depr     | Depreciation / PP&E                        | Holthausen & Larcker                         | 1992, JAE     | Compustat      | Annual    |
| 27  | divi     | Dividend initiation                        | Michaely, Thaler & Womack                    | 1995, JF      | Compustat      | Annual    |
| 28  | divo     | Dividend omission                          | Michaely, Thaler & Womack                    | 1995, JF      | Compustat      | Annual    |
| 29  | dolvol   | Dollar trading volume                      | Chordia, Subrahmanyam & Anshuman             | 2001, JFE     | CRSP           | Monthly   |
| 30  | dy       | Dividend to price                          | Litzenberger & Ramaswamy                     | 1982, JF      | Compustat      | Annual    |
| 31  | ear      | Earnings announcement return               | Kishore, Brandt, Santa-Clara & Venkatachalam | 2008, WP      | Compustat+CRSP | Quarterly |

Note: This table lists the characteristics we use in the empirical study. The data are collected in [Green et al. \(2017\)](#).

Table A.6: Details of the Characteristics (Continued)

| No. | Acronym         | Firm characteristic                                | Paper's author(s)                 | Year, Journal | Data Source | Frequency |
|-----|-----------------|----------------------------------------------------|-----------------------------------|---------------|-------------|-----------|
| 32  | egr             | Growth in common shareholder equity                | Richardson, Sloan, Soliman & Tuna | 2005, JAE     | Compustat   | Annual    |
| 33  | ep              | Earnings to price                                  | Basu                              | 1977, JF      | Compustat   | Annual    |
| 34  | gma             | Gross profitability                                | Novy-Marx                         | 2013, JFE     | Compustat   | Annual    |
| 35  | grCAPX          | Growth in capital expenditures                     | Anderson & Garcia-Feijoo          | 2006, JF      | Compustat   | Annual    |
| 36  | grltnoa         | Growth in long term net operating assets           | Fairfield, Whisenant & Yohn       | 2003, TAR     | Compustat   | Annual    |
| 37  | herf            | Industry sales concentration                       | Hou & Robinson                    | 2006, JF      | Compustat   | Annual    |
| 38  | hire            | Employee growth rate                               | Bazdresch, Belo & Lin             | 2014, JPE     | Compustat   | Annual    |
| 39  | idiovol         | Idiosyncratic return volatility                    | Ali, Hwang & Trombley             | 2003, JFE     | CRSP        | Monthly   |
| 40  | ill             | Illiquidity                                        | Amihud                            | 2002, JFM     | CRSP        | Monthly   |
| 41  | indmom          | Industry momentum                                  | Moskowitz & Grinblatt             | 1999, JF      | CRSP        | Monthly   |
| 42  | invest          | Capital expenditures and inventory                 | Chen & Zhang                      | 2010, JF      | Compustat   | Annual    |
| 43  | lev             | Leverage                                           | Bhandari                          | 1988, JF      | Compustat   | Annual    |
| 44  | lgr             | Growth in long-term debt                           | Richardson, Sloan, Soliman & Tuna | 2005, JAE     | Compustat   | Annual    |
| 45  | maxret          | Maximum daily return                               | Bali, Cakici & Whitelaw           | 2011, JFE     | CRSP        | Monthly   |
| 46  | mom12m          | 12-month momentum                                  | Jegadeesh                         | 1990, JF      | CRSP        | Monthly   |
| 47  | mom1m           | 1-month momentum                                   | Jegadeesh & Titman                | 1993, JF      | CRSP        | Monthly   |
| 48  | mom36m          | 36-month momentum                                  | Jegadeesh & Titman                | 1993, JF      | CRSP        | Monthly   |
| 49  | mom6m           | 6-month momentum                                   | Jegadeesh & Titman                | 1993, JF      | CRSP        | Monthly   |
| 50  | ms              | Financial statement score                          | Mohanram                          | 2005, RAS     | Compustat   | Quarterly |
| 51  | mvel1           | Size                                               | Banz                              | 1981, JFE     | CRSP        | Monthly   |
| 52  | mve1a           | Industry-adjusted size                             | Asness, Porter & Stevens          | 2000, WP      | Compustat   | Annual    |
| 53  | nincr           | Number of earnings increases                       | Barth, Elliott & Finn             | 1999, JAR     | Compustat   | Quarterly |
| 54  | operprof        | Operating profitability                            | Fama & French                     | 2015, JFE     | Compustat   | Annual    |
| 55  | orgcap          | Organizational capital                             | Eisfeldt & Papanikolaou           | 2013, JF      | Compustat   | Annual    |
| 56  | pchcapx1a       | Industry adjusted % change in capital expenditures | Abarbanell & Bushee               | 1998, TAR     | Compustat   | Annual    |
| 57  | pchcurrat       | % change in current ratio                          | Ou & Penman                       | 1989, JAE     | Compustat   | Annual    |
| 58  | pchdepr         | % change in depreciation                           | Holthausen & Larcker              | 1992, JAE     | Compustat   | Annual    |
| 59  | pchgm-pchsale   | % change in gross margin - % change in sales       | Abarbanell & Bushee               | 1998, TAR     | Compustat   | Annual    |
| 60  | pchquick        | % change in quick ratio                            | Ou & Penman                       | 1989, JAE     | Compustat   | Annual    |
| 61  | pchsale.pchinvt | % change in sales - % change in inventory          | Abarbanell & Bushee               | 1998, TAR     | Compustat   | Annual    |
| 62  | pchsale.pchrect | % change in sales - % change in A/R                | Abarbanell & Bushee               | 1998, TAR     | Compustat   | Annual    |

Table A.6: Details of the Characteristics (Continued)

| No. | Acronym         | Firm characteristic                             | Paper's author(s)                  | Year, Journal | Data Source | Frequency |
|-----|-----------------|-------------------------------------------------|------------------------------------|---------------|-------------|-----------|
| 63  | pchsale-pchxsga | % change in sales - % change in SG&A            | Abarbanell & Bushee                | 1998, TAR     | Compustat   | Annual    |
| 64  | pchsaleinv      | % change sales-to-inventory                     | Ou & Penman                        | 1989, JAE     | Compustat   | Annual    |
| 65  | ptacc           | Percent accruals                                | Hafzalla, Lundholm & Van Winkle    | 2011, TAR     | Compustat   | Annual    |
| 66  | pricedelay      | Price delay                                     | Hou & Moskowitz                    | 2005, RFS     | CRSP        | Monthly   |
| 67  | ps              | Financial statements score                      | Piotroski                          | 2000, JAR     | Compustat   | Annual    |
| 68  | quick           | Quick ratio                                     | Ou & Penman                        | 1989, JAE     | Compustat   | Annual    |
| 69  | rd              | R&D increase                                    | Eberhart, Maxwell & Siddique       | 2004, JF      | Compustat   | Annual    |
| 70  | rd_mve          | R&D to market capitalization                    | Guo, Lev & Shi                     | 2006, JBFA    | Compustat   | Annual    |
| 71  | rd_sale         | R&D to sales                                    | Guo, Lev & Shi                     | 2006, JBFA    | Compustat   | Annual    |
| 72  | realestate      | Real estate holdings                            | Tuzel                              | 2010, RFS     | Compustat   | Annual    |
| 73  | retvol          | Return volatility                               | Ang, Hodrick, King & Zhang         | 2006, JF      | CRSP        | Monthly   |
| 74  | roaq            | Return on assets                                | Balakrishnan, Bartov & Faurel      | 2010, JAE     | Compustat   | Quarterly |
| 75  | roavol          | Earnings volatility                             | Francis, LaFond, Olsson & Schipper | 2004, TAR     | Compustat   | Quarterly |
| 76  | roeq            | Return on equity                                | Hou, Xue & Zhang                   | 2015, RFS     | Compustat   | Quarterly |
| 77  | roic            | Return on invested capital                      | Brown & Rowe                       | 2007, WP      | Compustat   | Annual    |
| 78  | rsup            | Revenue surprise                                | Kama                               | 2009, JBFA    | Compustat   | Quarterly |
| 79  | salecash        | Sales to cash                                   | Ou & Penman                        | 1989, JAE     | Compustat   | Annual    |
| 80  | saleinv         | Sales to inventory                              | Ou & Penman                        | 1989, JAE     | Compustat   | Annual    |
| 81  | salerec         | Sales to receivables                            | Ou & Penman                        | 1989, JAE     | Compustat   | Annual    |
| 82  | secured         | Secured debt                                    | Valta                              | 2016, JFQA    | Compustat   | Annual    |
| 83  | securedind      | Secured debt indicator                          | Valta                              | 2016, JFQA    | Compustat   | Annual    |
| 84  | sg              | Sales growth                                    | Lakonishok, Shleifer & Vishny      | 1994, JF      | Compustat   | Annual    |
| 85  | sin             | Sin stocks                                      | Hong & Kacperczyk                  | 2009, JFE     | Compustat   | Annual    |
| 86  | sp              | Sales to price                                  | Barbee, Mukherji, & Raines         | 1996, FAJ     | Compustat   | Annual    |
| 87  | std_dolvol      | Volatility of liquidity (dollar trading volume) | Chordia, Subrahmanyam & Anshuman   | 2001, JFE     | CRSP        | Monthly   |
| 88  | std_turn        | Volatility of liquidity (share turnover)        | Chordia, Subrahmanyam, & Anshuman  | 2001, JFE     | CRSP        | Monthly   |
| 89  | stdacc          | Accrual volatility                              | Bandyopadhyay, Huang & Wirjanto    | 2010, WP      | Compustat   | Quarterly |
| 90  | stdcf           | Cash flow volatility                            | Huang                              | 2009, JEF     | Compustat   | Quarterly |
| 91  | tang            | Debt capacity/firm tangibility                  | Almeida & Campello                 | 2007, RFS     | Compustat   | Annual    |
| 92  | tb              | Tax income to book income                       | Lev & Nissim                       | 2004, TAR     | Compustat   | Annual    |
| 93  | turn            | Share turnover                                  | Datar, Naik & Radcliffe            | 1998, JFM     | Compustat   | Monthly   |
| 94  | zerotrade       | Zero trading days                               | Liu                                | 2006, JFE     | CRSP        | Monthly   |

Table A.7: Implied Sharpe Ratio Improvements

|                                              | OLS-3<br>+H | PLS  | PCR  | ENet<br>+H | GLM<br>+H | RF   | GBRT<br>+H | NN1  | NN2  | NN3  | NN4  | NN5  |
|----------------------------------------------|-------------|------|------|------------|-----------|------|------------|------|------|------|------|------|
| Panel A: Common Factor Portfolios            |             |      |      |            |           |      |            |      |      |      |      |      |
| S&P 500                                      | -           | -    | -    | 0.08       | 0.08      | 0.14 | 0.15       | 0.11 | 0.12 | 0.20 | 0.17 | 0.12 |
| SMB                                          | 0.2         | 0.39 | 0.12 | 0.34       | 0.42      | 0.16 | 0.11       | 0.30 | 0.26 | 0.28 | 0.27 | 0.28 |
| HML                                          | 0.12        | 0.09 | 0.20 | 0.09       | 0.15      | 0.17 | 0.04       | 0.20 | 0.21 | 0.18 | 0.20 | 0.20 |
| RMW                                          | -           | 0.15 | 0.06 | -          | -         | -    | -          | 0.9  | 0.06 | 0.11 | 0.07 | 0.07 |
| CMA                                          | 0.10        | -    | 0.00 | -          | 0.14      | -    | -          | 0.20 | 0.18 | 0.12 | 0.20 | 0.15 |
| UMD                                          | -           | -    | -    | 0.12       | -         | 0.27 | -          | -    | -    | 0.06 | 0.08 | 0.10 |
| Panel B: Sub-components of Factor Portfolios |             |      |      |            |           |      |            |      |      |      |      |      |
| Big Value                                    | 0.05        | 0.00 | -    | 0.03       | 0.07      | 0.14 | 0.12       | 0.09 | 0.10 | 0.15 | 0.13 | 0.11 |
| Big Growth                                   | -           | -    | -    | 0.08       | 0.06      | 0.14 | 0.13       | 0.11 | 0.12 | 0.16 | 0.13 | 0.12 |
| Big Neutral                                  | 0.01        | -    | -    | 0.08       | 0.04      | 0.13 | 0.13       | 0.15 | 0.13 | 0.17 | 0.18 | 0.14 |
| Small Value                                  | 0.02        | 0.15 | 0.10 | 0.06       | 0.08      | 0.11 | 0.05       | 0.14 | 0.13 | 0.14 | 0.13 | 0.12 |
| Small Growth                                 | -           | 0.03 | -    | -          | -         | 0.14 | 0.21       | 0.01 | 0.09 | 0.10 | 0.08 | 0.10 |
| Small Neutral                                | -           | 0.06 | 0.02 | 0.02       | 0.03      | 0.09 | 0.04       | 0.06 | 0.06 | 0.07 | 0.06 | 0.07 |
| Big Conservative                             | -           | -    | -    | 0.09       | 0.04      | 0.10 | 0.05       | 0.11 | 0.10 | 0.14 | 0.12 | 0.10 |
| Big Aggressive                               | -           | -    | -    | 0.04       | 0.09      | 0.20 | 0.23       | 0.16 | 0.18 | 0.21 | 0.18 | 0.17 |
| Big Neutral                                  | -           | -    | -    | 0.08       | 0.05      | 0.11 | 0.08       | 0.08 | 0.08 | 0.14 | 0.14 | 0.11 |
| Small Conservative                           | -           | 0.12 | 0.08 | 0.00       | 0.04      | 0.10 | 0.06       | 0.09 | 0.09 | 0.10 | 0.09 | 0.09 |
| Small Aggressive                             | -           | 0.09 | 0.00 | -          | 0.03      | 0.16 | 0.22       | 0.06 | 0.11 | 0.12 | 0.10 | 0.12 |
| Small Neutral                                | -           | 0.04 | 0.01 | 0.04       | 0.03      | 0.07 | 0.00       | 0.06 | 0.06 | 0.08 | 0.06 | 0.07 |
| Big Robust                                   | -           | -    | -    | 0.06       | 0.04      | 0.11 | 0.03       | 0.08 | 0.08 | 0.13 | 0.10 | 0.08 |
| Big Weak                                     | 0.03        | 0.15 | 0.12 | 0.10       | 0.12      | 0.14 | 0.19       | 0.19 | 0.19 | 0.21 | 0.17 | 0.17 |
| Big Neutral                                  | -           | -    | -    | 0.06       | 0.02      | 0.14 | 0.12       | 0.11 | 0.13 | 0.15 | 0.15 | 0.13 |
| Small Robust                                 | -           | 0.04 | -    | 0.00       | -         | 0.07 | 0.02       | 0.02 | 0.05 | 0.06 | 0.05 | 0.05 |
| Small Weak                                   | 0.04        | 0.17 | 0.11 | -          | 0.08      | 0.17 | 0.22       | 0.13 | 0.15 | 0.16 | 0.15 | 0.15 |
| Small Neutral                                | -           | 0.01 | -    | -          | -         | 0.06 | -          | 0.01 | 0.03 | 0.04 | 0.03 | 0.04 |
| Big Up                                       | -           | -    | -    | 0.06       | 0.11      | 0.11 | 0.08       | 0.07 | 0.07 | 0.10 | 0.10 | 0.09 |
| Big Down                                     | -           | -    | -    | 0.05       | -         | 0.13 | 0.08       | 0.04 | 0.08 | 0.12 | 0.10 | 0.10 |
| Big Medium                                   | -           | -    | -    | 0.13       | -         | 0.22 | 0.25       | 0.19 | 0.20 | 0.24 | 0.22 | 0.18 |
| Small Up                                     | -           | 0.08 | 0.06 | -          | 0.03      | 0.07 | 0.00       | 0.01 | 0.01 | 0.02 | 0.02 | 0.03 |
| Small Down                                   | -           | 0.03 | -    | 0.03       | 0.00      | 0.23 | 0.22       | 0.13 | 0.14 | 0.17 | 0.15 | 0.16 |
| Small Medium                                 | 0.01        | 0.08 | 0.02 | 0.06       | 0.04      | 0.12 | 0.11       | 0.11 | 0.11 | 0.12 | 0.10 | 0.10 |

Note: Improvement in annualized Sharpe ratio ( $SR^* - SR$ ) implied by the full sample Sharpe ratio of each portfolio together with machine learning predictive  $R^2_{\text{os}}$  from Table 5. Cases with negative  $R^2_{\text{os}}$  imply a Sharpe ratio deterioration and are omitted.

Figure A.1: Characteristic Importance over Time by NN3

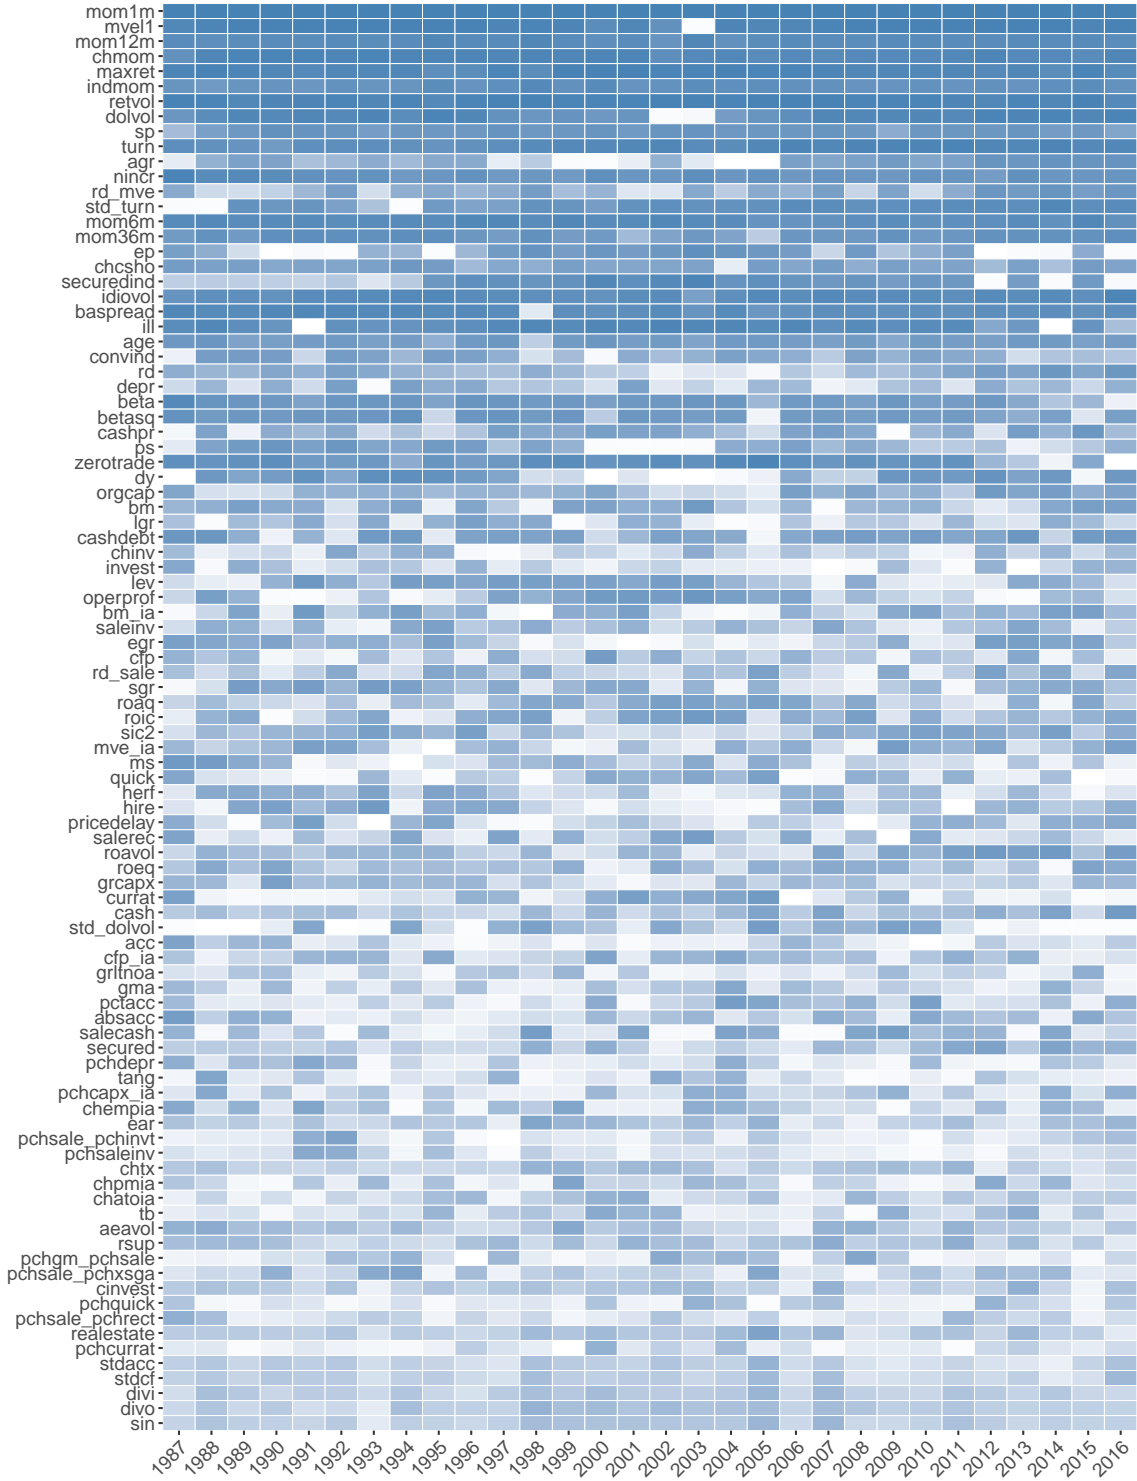

Note: This figure describes how NN3 ranks the 94 stock-level characteristics and the industry dummy (sic2) in terms of overall model contribution over 30 recurring training. Columns correspond to the year end of each of the 30 samples, and color gradients within each column indicate the most influential (dark blue) to least influential (white) variables. Characteristics are sorted in the same order of Figure 5.



Figure A.3: Characteristic Importance with Placebo Variables

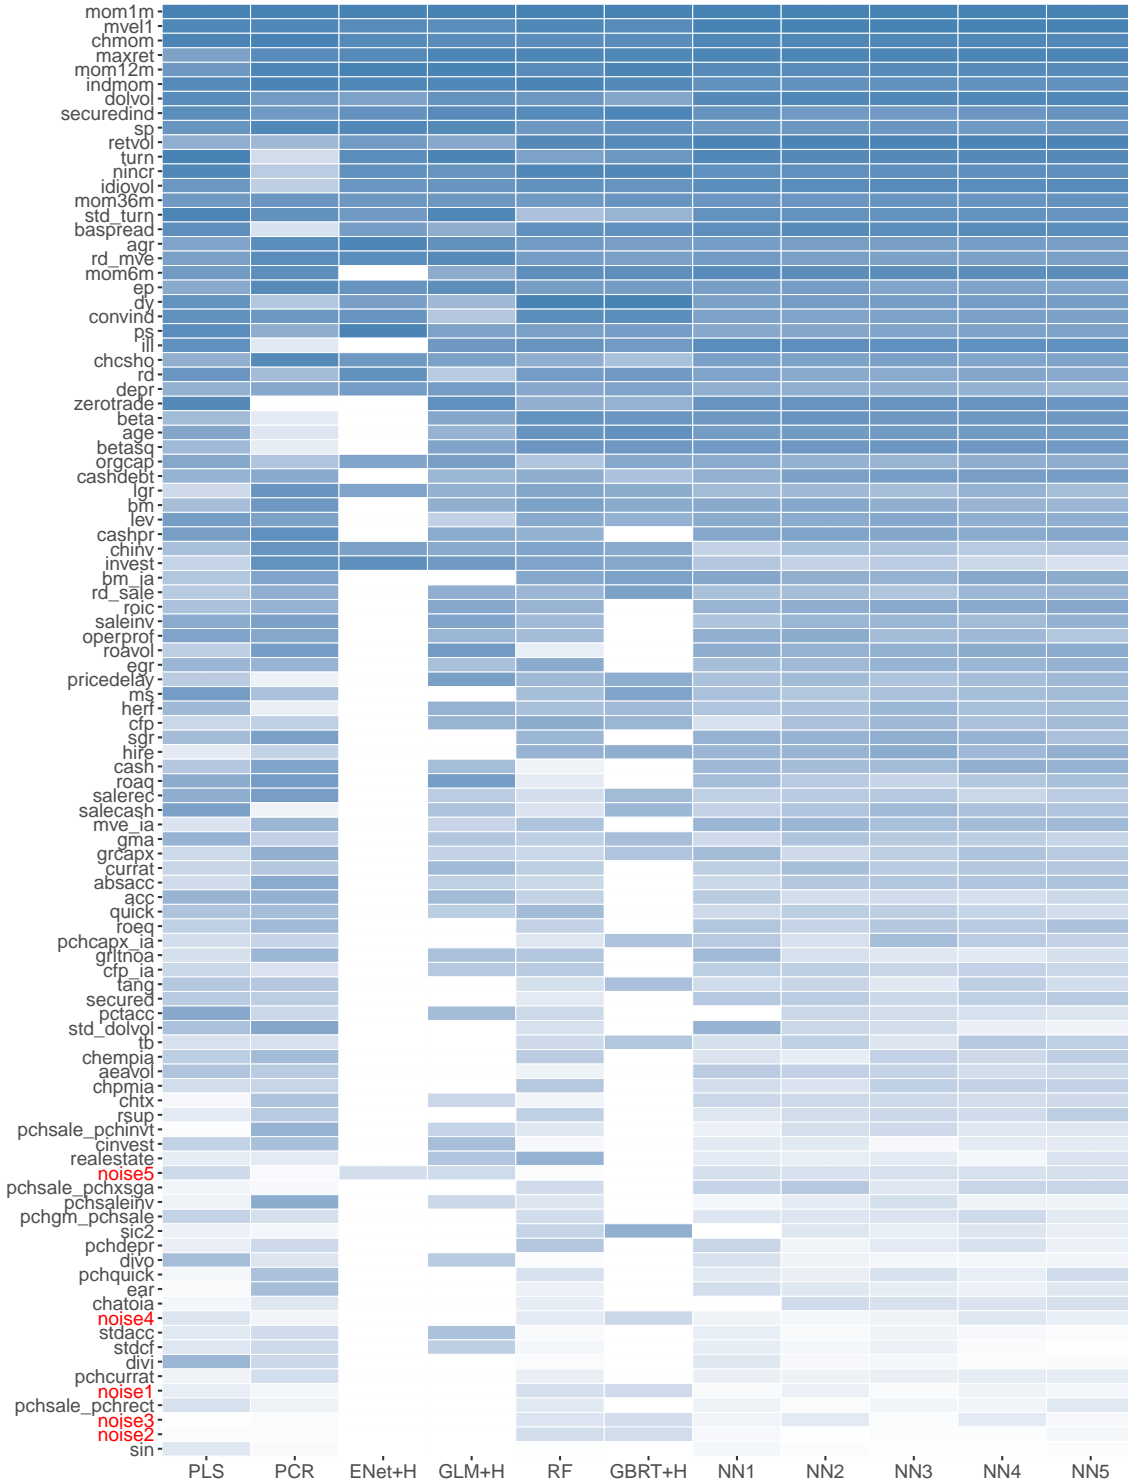

Note: This figure describes how each model ranks the 94 stock-level characteristics, the industry dummy (sic2), and five placebos in terms of overall model contribution. Columns correspond to individual models, and color gradients within each column indicate the most influential (dark blue) to least influential (white) variables. Characteristics are ordered based on the sum of their ranks over all models, with the most influential characteristics on top and least influential on bottom.

Figure A.4: Stock/Macroeconomic Interactions

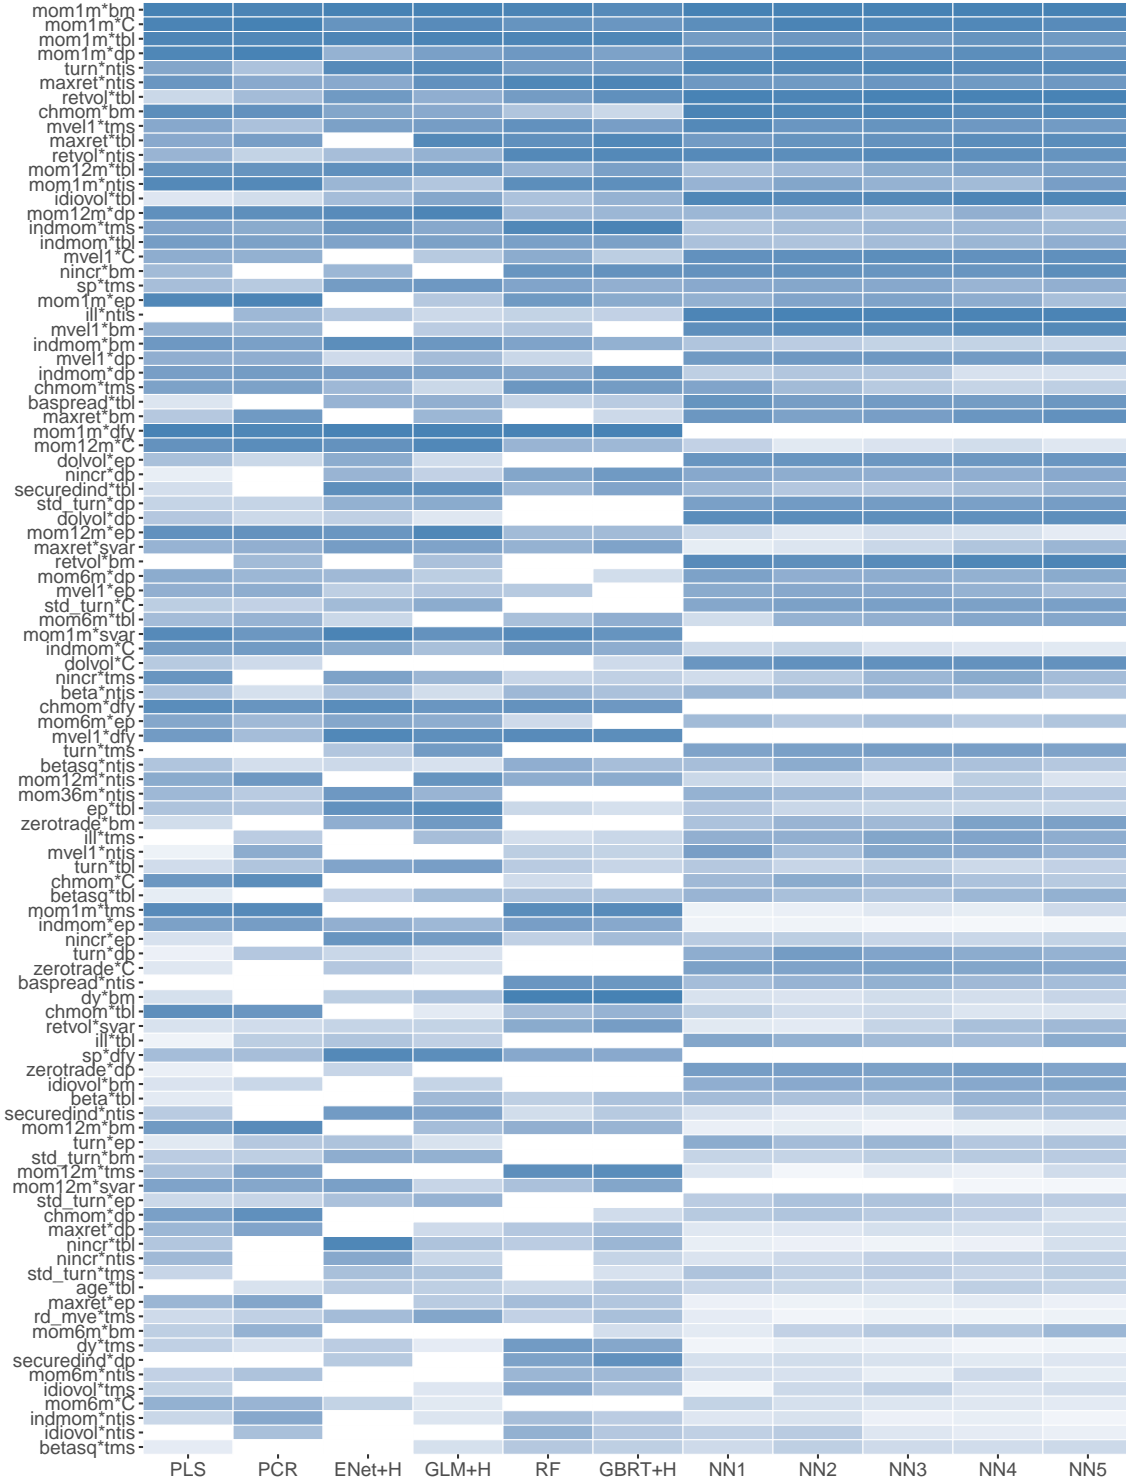

Note: Rankings of top 100 interactions between 94 stock-level stock characteristics and nine macro variables (including a constant, denoted  $C$ ). Interactions are ordered based on the sum of their ranks over all models, with the most influential characteristics on top and least influential on bottom. Columns correspond to individual models, and color gradients within each column indicate the most influential (dark blue) to least influential (white) interactions.

Figure A.5: Time Variation in Stock/Macroeconomic Interactions

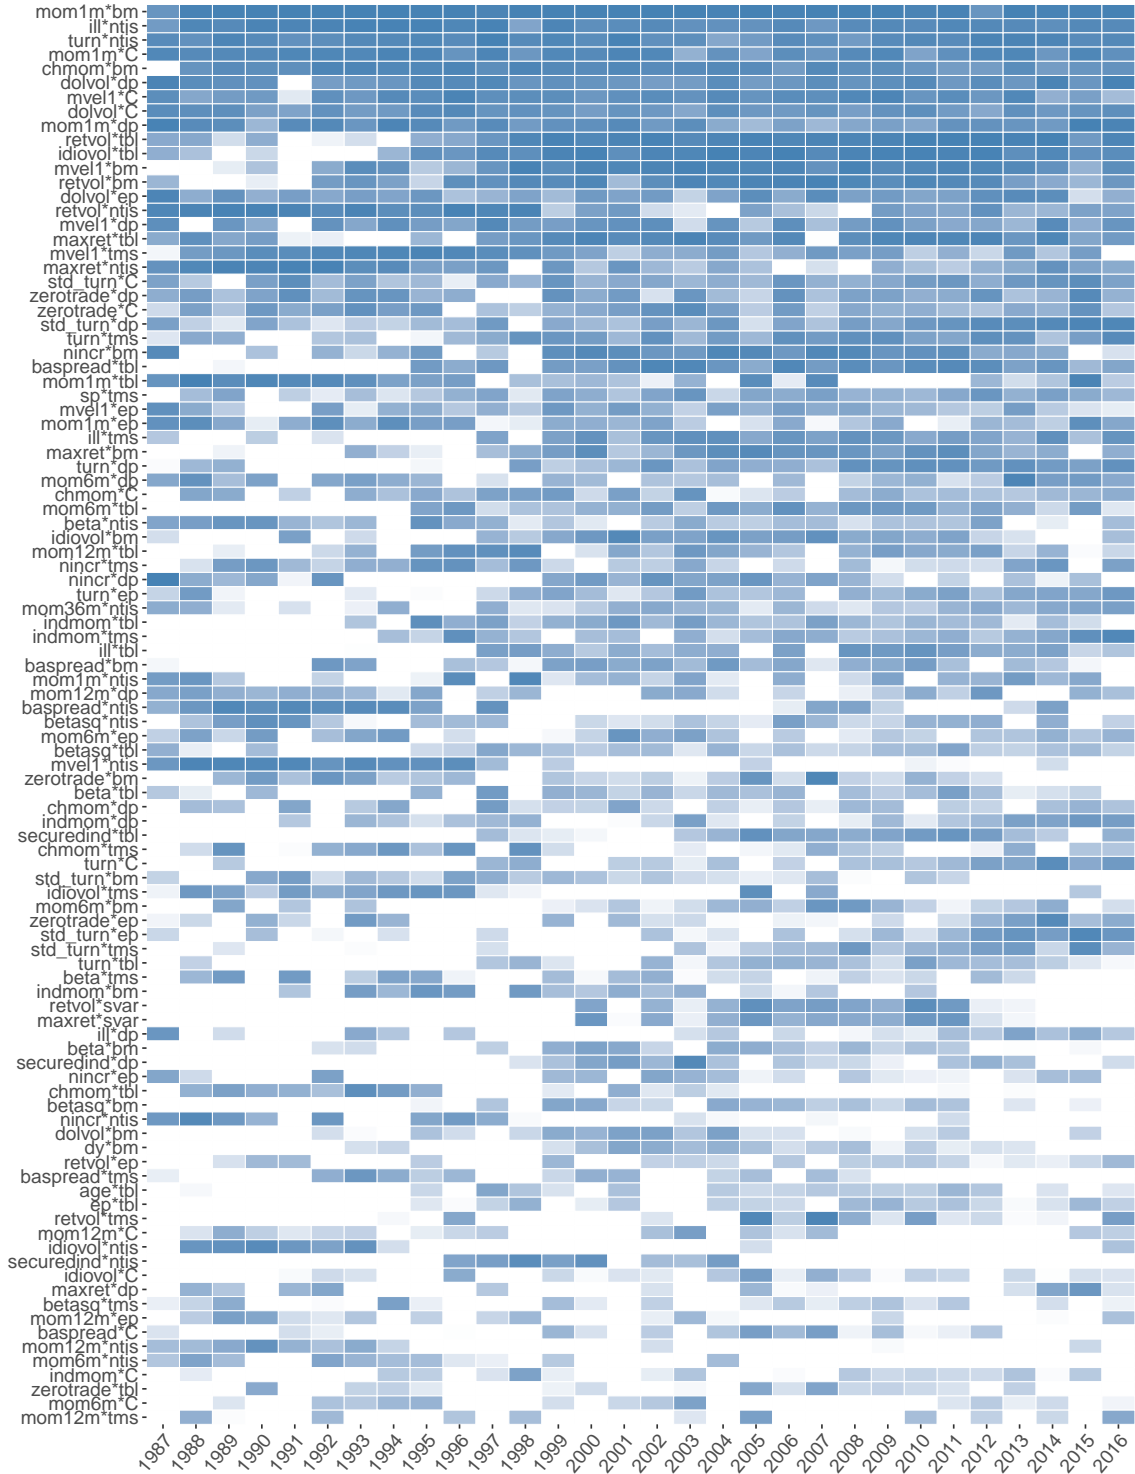

Note: Rankings of top 100 interactions between 94 stock-level stock characteristics and nine macro variables (including a constant, denoted  $C$ ). The list of top 100 interactions is based on the analysis in Figure A.4. Color gradients indicate the most influential (dark blue) to least influential (white) interactions in the NN3 model in each training sample (the horizontal axis corresponds to the last year in each training sample).

Figure A.6: Characteristic Importance at Annual Horizon

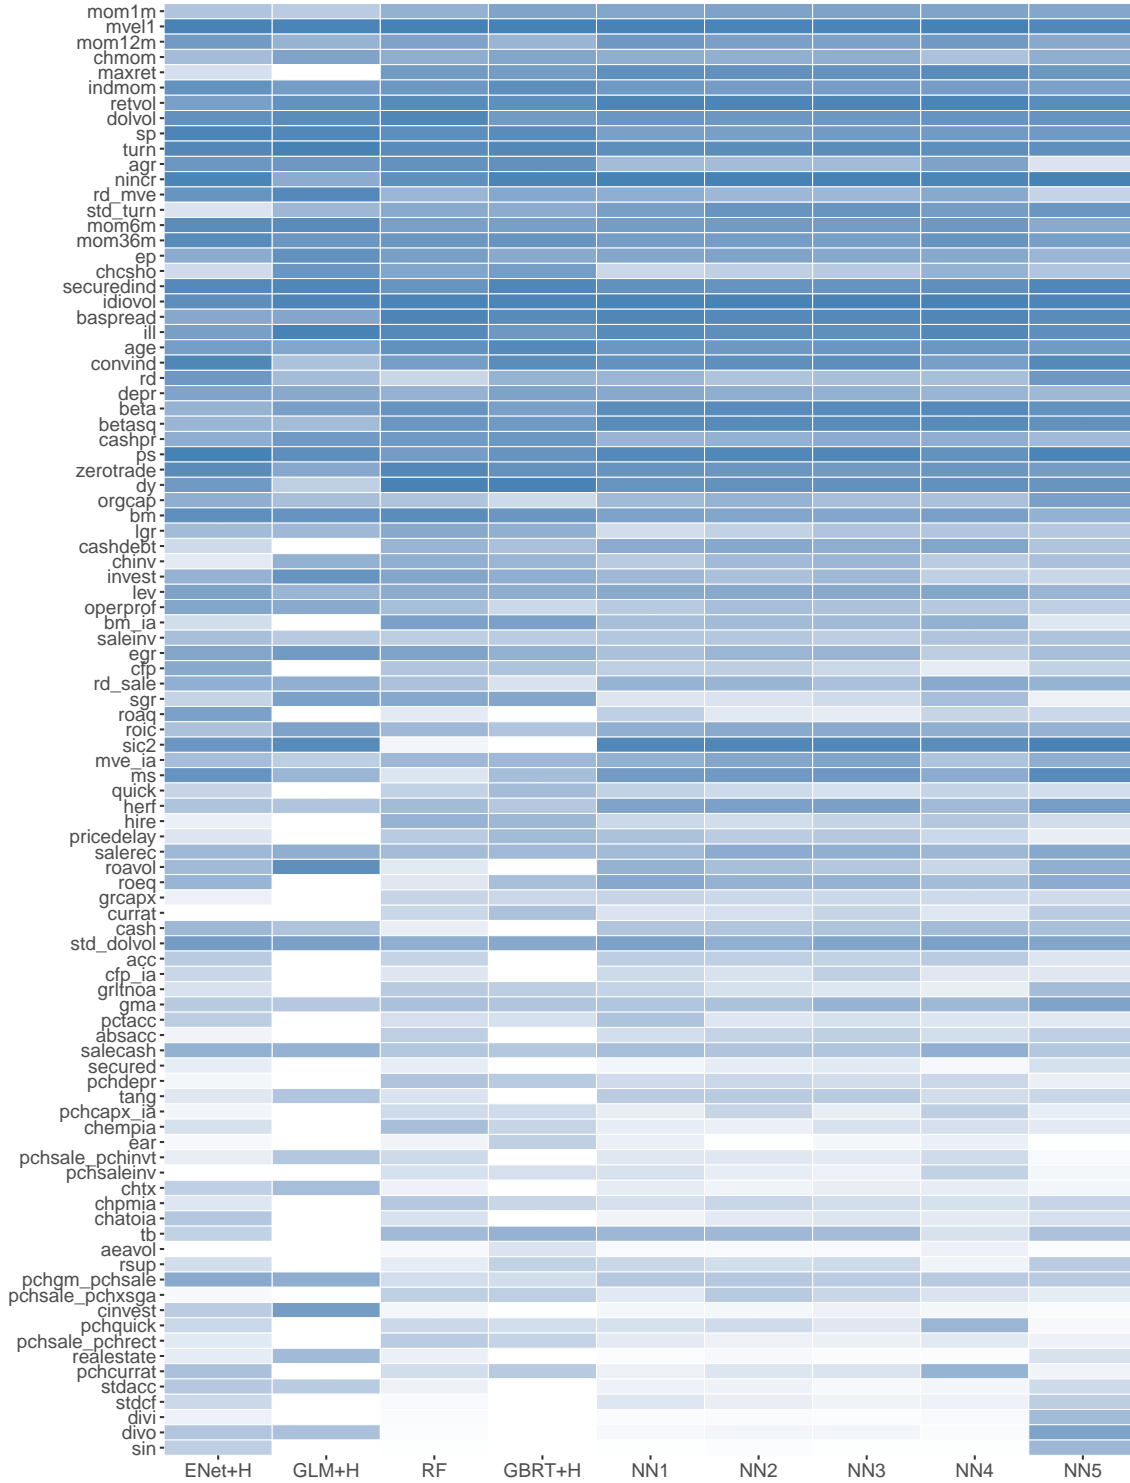

Note: This figure describes how each model ranks the 94 stock-level characteristics and the industry dummy (sic2) in terms of overall model contribution. Columns correspond to individual models, and color gradients within each column indicate the most influential (dark blue) to least influential (white) variables. Characteristic gradients within each order of Figure 5. The results are based on prediction at the annual horizon.

Table A.8: Annual Portfolio-level Out-of-Sample Predictive  $R^2$ 

|                                              | OLS-3<br>+H | PLS    | PCR    | ENet<br>+H | GLM<br>+H | RF    | GBRT<br>+H | NN1    | NN2   | NN3   | NN4   | NN5   |
|----------------------------------------------|-------------|--------|--------|------------|-----------|-------|------------|--------|-------|-------|-------|-------|
| Panel A: Common Factor Portfolios            |             |        |        |            |           |       |            |        |       |       |       |       |
| S&P 500                                      | -4.90       | 0.43   | -7.17  | 0.26       | 2.07      | 8.80  | 7.28       | 9.99   | 12.02 | 15.68 | 15.30 | 13.15 |
| SMB                                          | 3.77        | 4.23   | 8.26   | 4.22       | 6.96      | 6.54  | 4.27       | 0.05   | 1.31  | 2.59  | 4.33  | 4.45  |
| HML                                          | 3.01        | -0.52  | 4.08   | -0.15      | 6.33      | 7.02  | 2.17       | 9.14   | 8.09  | 7.86  | 3.97  | 3.63  |
| RMW                                          | 4.66        | 17.11  | 6.67   | 1.19       | 3.45      | 3.51  | 5.31       | 7.03   | 5.03  | 3.58  | 0.61  | 0.90  |
| CMA                                          | 4.50        | -1.52  | 7.94   | -9.01      | 7.69      | 1.73  | -8.36      | 5.89   | 7.27  | 0.93  | -7.18 | -8.11 |
| UMD                                          | -27.52      | -12.44 | -5.62  | -16.27     | -8.06     | -7.57 | -8.29      | -12.78 | -8.71 | -7.35 | -6.45 | -6.74 |
| Panel B: Sub-components of Factor Portfolios |             |        |        |            |           |       |            |        |       |       |       |       |
| Big Value                                    | 1.83        | 4.88   | -4.04  | 3.62       | 0.49      | 9.50  | 5.86       | 8.76   | 8.54  | 12.42 | 9.95  | 7.56  |
| Big Growth                                   | -12.06      | -6.92  | -10.22 | -2.13      | 2.44      | 7.14  | 6.93       | 7.47   | 11.06 | 11.67 | 13.37 | 10.03 |
| Big Neutral                                  | -3.83       | 3.09   | -6.58  | 1.19       | 1.24      | 8.52  | 6.91       | 8.31   | 11.51 | 14.60 | 12.92 | 9.95  |
| Small Value                                  | 4.31        | 10.81  | 8.94   | 8.41       | 4.31      | 8.05  | 3.75       | 7.24   | 6.37  | 7.48  | 6.60  | 4.81  |
| Small Growth                                 | 2.49        | 2.87   | 3.19   | 0.21       | 0.03      | 6.20  | 2.13       | 3.96   | 5.52  | 6.84  | 2.60  | 7.23  |
| Small Neutral                                | -1.52       | 5.21   | 2.10   | 2.29       | 2.29      | 4.18  | 1.78       | 6.46   | 5.55  | 6.68  | 3.69  | 6.14  |
| Big Conservative                             | -10.42      | -2.42  | -9.77  | -3.77      | 5.17      | 8.44  | 5.26       | -1.31  | 8.64  | 9.65  | 12.47 | 6.09  |
| Big Aggressive                               | -1.65       | 1.89   | -4.72  | 1.36       | 2.00      | 7.42  | 6.67       | 11.00  | 11.74 | 13.08 | 11.27 | 10.67 |
| Big Neutral                                  | -9.18       | -1.62  | -9.42  | 2.03       | 2.43      | 9.62  | 8.39       | 10.88  | 13.03 | 15.61 | 15.75 | 13.56 |
| Small Conservative                           | -0.38       | 6.36   | 5.01   | 3.19       | 2.35      | 4.60  | 0.62       | 5.31   | 5.39  | 5.97  | 4.22  | 4.71  |
| Small Aggressive                             | 3.33        | 5.12   | 2.88   | 1.04       | 0.37      | 6.43  | 3.23       | 2.50   | 4.50  | 5.50  | 1.47  | 6.56  |
| Small Neutral                                | -0.53       | 5.84   | 3.52   | 4.46       | 3.59      | 7.08  | 2.96       | 8.41   | 7.13  | 8.68  | 5.77  | 8.47  |
| Big Robust                                   | -7.53       | -2.55  | -9.18  | 1.33       | 5.42      | 7.61  | 6.60       | 12.55  | 12.04 | 13.92 | 15.29 | 13.35 |
| Big Weak                                     | -3.40       | 3.09   | -7.15  | -1.02      | -1.12     | 9.62  | 7.62       | 4.41   | 9.95  | 11.39 | 11.73 | 8.40  |
| Big Neutral                                  | -4.17       | 5.46   | -4.57  | -3.18      | -2.12     | 6.24  | 4.47       | 4.18   | 6.23  | 9.47  | 3.70  | 2.95  |
| Small Robust                                 | -2.37       | 0.93   | -0.20  | 0.76       | 3.72      | 0.41  | -0.87      | 2.92   | 3.67  | 4.47  | 0.86  | 4.19  |
| Small Weak                                   | 3.88        | 9.89   | 5.68   | 2.15       | -1.11     | 7.53  | 3.10       | -0.48  | 1.53  | 2.96  | 1.61  | 1.08  |
| Small Neutral                                | 3.00        | 7.99   | 4.40   | 4.60       | 3.58      | 9.21  | 5.75       | 10.03  | 7.39  | 9.82  | 7.06  | 9.09  |
| Big Up                                       | -23.55      | -11.77 | -19.16 | -5.11      | 0.52      | 6.15  | 6.21       | 4.26   | 11.44 | 11.11 | 14.48 | 10.62 |
| Big Down                                     | -4.66       | 0.39   | -2.79  | -0.15      | 0.71      | 7.64  | 5.53       | 3.58   | 8.78  | 9.54  | 10.32 | 6.79  |
| Big Medium                                   | 6.26        | 10.24  | 7.36   | 6.25       | 3.83      | 7.73  | 5.38       | 8.74   | 9.61  | 11.36 | 9.96  | 6.22  |
| Small Up                                     | -6.68       | 3.82   | 0.71   | -2.83      | 1.57      | 1.84  | -0.19      | -4.22  | 0.70  | 1.12  | -1.42 | 2.83  |
| Small Down                                   | 2.80        | 5.59   | 4.84   | 2.87       | 0.50      | 7.23  | 3.49       | 3.24   | 4.63  | 5.90  | 3.28  | 5.22  |
| Small Medium                                 | -2.92       | -0.49  | -1.70  | -1.80      | 0.81      | 2.00  | -0.40      | -1.64  | 1.96  | 1.79  | 0.51  | 3.49  |

Note: In this table, we report the out-of-sample predictive  $R^2$ s for 30 portfolios using OLS with size, book-to-market, and momentum, OLS-3, PLS, PCR, elastic net (ENet), generalized linear model with group lasso (GLM), random forest (RF), gradient boosted regression trees (GBRT), and five architectures of neural networks (NN1,...,NN5), respectively. “+H” indicates the use of Huber loss instead of the  $l_2$  loss. The six portfolios in Panel A are the S&P 500 index and the Fama-French SMB, HML, CMA, RMW, and UMD factors. The 24 portfolios in Panel B are  $3 \times 2$  size double-sorted portfolios used in the construction of the Fama-French value, investment, profitability, and momentum factors. The results are based on prediction at the annual horizon.

Table A.9: Performance of Machine Learning Portfolios (Equally Weighted)

|         | OLS-3+H |       |      |       | PLS   |       |      |       | PCR   |       |      |       |
|---------|---------|-------|------|-------|-------|-------|------|-------|-------|-------|------|-------|
|         | Pred    | Avg   | Std  | SR    | Pred  | Avg   | Std  | SR    | Pred  | Avg   | Std  | SR    |
| Low(L)  | -0.14   | 0.11  | 7.99 | 0.05  | -0.83 | -0.26 | 6.41 | -0.14 | -0.71 | -0.65 | 7.04 | -0.32 |
| 2       | 0.17    | 0.35  | 6.81 | 0.18  | -0.20 | 0.19  | 5.92 | 0.11  | -0.11 | 0.16  | 6.23 | 0.09  |
| 3       | 0.35    | 0.44  | 6.09 | 0.25  | 0.12  | 0.40  | 5.49 | 0.25  | 0.19  | 0.40  | 5.67 | 0.25  |
| 4       | 0.49    | 0.63  | 5.61 | 0.39  | 0.39  | 0.67  | 5.06 | 0.46  | 0.42  | 0.58  | 5.45 | 0.37  |
| 5       | 0.63    | 0.73  | 5.24 | 0.49  | 0.62  | 0.69  | 5.14 | 0.47  | 0.63  | 0.72  | 5.11 | 0.49  |
| 6       | 0.75    | 0.83  | 4.88 | 0.59  | 0.84  | 0.77  | 5.14 | 0.52  | 0.81  | 0.80  | 4.98 | 0.55  |
| 7       | 0.88    | 0.75  | 4.73 | 0.55  | 1.06  | 0.88  | 5.12 | 0.60  | 1.01  | 0.98  | 5.02 | 0.68  |
| 8       | 1.03    | 0.80  | 4.72 | 0.59  | 1.32  | 1.01  | 5.29 | 0.66  | 1.23  | 1.08  | 5.02 | 0.75  |
| 9       | 1.22    | 1.14  | 4.73 | 0.83  | 1.67  | 1.28  | 5.60 | 0.79  | 1.52  | 1.33  | 5.28 | 0.88  |
| High(H) | 1.60    | 1.45  | 5.21 | 0.96  | 2.38  | 1.82  | 6.16 | 1.02  | 2.12  | 1.81  | 5.93 | 1.06  |
| H-L     | 1.73    | 1.34  | 5.59 | 0.83  | 3.21  | 2.08  | 4.89 | 1.47  | 2.83  | 2.45  | 4.51 | 1.89  |
|         | ENet+H  |       |      |       | GLM+H |       |      |       | RF    |       |      |       |
|         | Pred    | Avg   | Std  | SR    | Pred  | Avg   | Std  | SR    | Pred  | Avg   | Std  | SR    |
| Low(L)  | -0.04   | -0.24 | 6.43 | -0.13 | -0.49 | -0.50 | 6.81 | -0.25 | 0.26  | -0.48 | 7.16 | -0.23 |
| 2       | 0.27    | 0.44  | 5.90 | 0.26  | 0.01  | 0.32  | 5.80 | 0.19  | 0.44  | 0.24  | 5.67 | 0.15  |
| 3       | 0.44    | 0.52  | 5.27 | 0.34  | 0.29  | 0.56  | 5.46 | 0.36  | 0.53  | 0.55  | 5.36 | 0.36  |
| 4       | 0.59    | 0.70  | 4.73 | 0.51  | 0.50  | 0.61  | 5.22 | 0.41  | 0.60  | 0.62  | 5.15 | 0.42  |
| 5       | 0.73    | 0.71  | 4.94 | 0.49  | 0.68  | 0.72  | 5.11 | 0.49  | 0.67  | 0.66  | 5.11 | 0.44  |
| 6       | 0.87    | 0.79  | 5.00 | 0.55  | 0.84  | 0.78  | 5.12 | 0.53  | 0.73  | 0.77  | 5.13 | 0.52  |
| 7       | 1.01    | 0.85  | 5.21 | 0.56  | 1.00  | 0.78  | 5.06 | 0.54  | 0.80  | 0.74  | 5.10 | 0.50  |
| 8       | 1.17    | 0.88  | 5.47 | 0.56  | 1.18  | 0.89  | 5.14 | 0.60  | 0.87  | 0.99  | 5.29 | 0.65  |
| 9       | 1.36    | 0.85  | 5.90 | 0.50  | 1.41  | 1.25  | 5.80 | 0.75  | 0.97  | 1.22  | 5.67 | 0.74  |
| High(H) | 1.72    | 1.86  | 7.27 | 0.89  | 1.89  | 1.81  | 6.57 | 0.96  | 1.20  | 1.90  | 7.03 | 0.94  |
| H-L     | 1.76    | 2.11  | 5.50 | 1.33  | 2.38  | 2.31  | 4.41 | 1.82  | 0.94  | 2.38  | 5.57 | 1.48  |
|         | GBRT+H  |       |      |       | NN1   |       |      |       | NN2   |       |      |       |
|         | Pred    | Avg   | Std  | SR    | Pred  | Avg   | Std  | SR    | Pred  | Avg   | Std  | SR    |
| Low(L)  | -0.49   | -0.37 | 6.46 | -0.20 | -0.45 | -0.78 | 7.43 | -0.36 | -0.32 | -1.01 | 7.79 | -0.45 |
| 2       | -0.16   | 0.42  | 5.80 | 0.25  | 0.15  | 0.22  | 6.24 | 0.12  | 0.20  | 0.17  | 6.34 | 0.09  |
| 3       | 0.02    | 0.56  | 5.31 | 0.36  | 0.43  | 0.47  | 5.55 | 0.29  | 0.43  | 0.52  | 5.49 | 0.33  |
| 4       | 0.17    | 0.74  | 5.43 | 0.47  | 0.64  | 0.64  | 5.00 | 0.45  | 0.59  | 0.71  | 5.02 | 0.49  |
| 5       | 0.33    | 0.63  | 5.31 | 0.41  | 0.80  | 0.80  | 4.76 | 0.58  | 0.72  | 0.76  | 4.60 | 0.57  |
| 6       | 0.46    | 0.83  | 5.23 | 0.55  | 0.95  | 0.85  | 4.63 | 0.63  | 0.84  | 0.81  | 4.52 | 0.62  |
| 7       | 0.59    | 0.67  | 5.13 | 0.45  | 1.12  | 0.84  | 4.66 | 0.62  | 0.97  | 0.94  | 4.61 | 0.70  |
| 8       | 0.72    | 0.82  | 5.08 | 0.56  | 1.32  | 0.88  | 4.95 | 0.62  | 1.14  | 0.92  | 4.86 | 0.66  |
| 9       | 0.88    | 1.12  | 5.41 | 0.72  | 1.63  | 1.17  | 5.62 | 0.72  | 1.41  | 1.10  | 5.55 | 0.69  |
| High(H) | 1.19    | 1.77  | 6.69 | 0.92  | 2.43  | 2.13  | 7.34 | 1.00  | 2.25  | 2.30  | 7.81 | 1.02  |
| H-L     | 1.68    | 2.14  | 4.28 | 1.73  | 2.89  | 2.91  | 4.72 | 2.13  | 2.57  | 3.31  | 4.92 | 2.33  |
|         | NN3     |       |      |       | NN4   |       |      |       | NN5   |       |      |       |
|         | Pred    | Avg   | Std  | SR    | Pred  | Avg   | Std  | SR    | Pred  | Avg   | Std  | SR    |
| Low(L)  | -0.31   | -0.92 | 7.94 | -0.40 | -0.19 | -0.95 | 7.83 | -0.42 | -0.08 | -0.83 | 7.92 | -0.36 |
| 2       | 0.22    | 0.16  | 6.46 | 0.09  | 0.29  | 0.17  | 6.50 | 0.09  | 0.33  | 0.24  | 6.64 | 0.12  |
| 3       | 0.45    | 0.44  | 5.40 | 0.28  | 0.49  | 0.45  | 5.58 | 0.28  | 0.51  | 0.53  | 5.65 | 0.32  |
| 4       | 0.60    | 0.66  | 4.83 | 0.48  | 0.62  | 0.57  | 4.94 | 0.40  | 0.62  | 0.59  | 4.91 | 0.41  |
| 5       | 0.73    | 0.77  | 4.58 | 0.58  | 0.72  | 0.70  | 4.57 | 0.53  | 0.71  | 0.68  | 4.56 | 0.51  |
| 6       | 0.85    | 0.81  | 4.47 | 0.63  | 0.81  | 0.75  | 4.42 | 0.59  | 0.80  | 0.76  | 4.43 | 0.60  |
| 7       | 0.97    | 0.86  | 4.62 | 0.64  | 0.91  | 0.86  | 4.47 | 0.67  | 0.88  | 0.88  | 4.60 | 0.66  |
| 8       | 1.12    | 0.93  | 4.82 | 0.67  | 1.04  | 1.06  | 4.82 | 0.76  | 1.01  | 0.95  | 4.90 | 0.67  |
| 9       | 1.38    | 1.18  | 5.51 | 0.74  | 1.28  | 1.24  | 5.57 | 0.77  | 1.25  | 1.17  | 5.60 | 0.73  |
| High(H) | 2.28    | 2.35  | 8.11 | 1.00  | 2.16  | 2.37  | 8.03 | 1.02  | 2.08  | 2.27  | 7.95 | 0.99  |
| H-L     | 2.58    | 3.27  | 4.80 | 2.36  | 2.35  | 3.33  | 4.71 | 2.45  | 2.16  | 3.09  | 4.98 | 2.15  |

Note: Performance of equal-weight decile portfolios sorted on out-of-sample machine learning return forecasts. “Pred”, “Avg”, “Std”, and “SR” report the predicted monthly returns for each decile, the average realized monthly returns, their realized standard deviations, and annualized Sharpe ratios, respectively.

Table A.10: Performance of Machine Learning Portfolios (Equally Weighted, Excluding Microcaps)

|         | OLS-3+H |       |      |       | PLS   |       |      |       | PCR   |       |      |       |
|---------|---------|-------|------|-------|-------|-------|------|-------|-------|-------|------|-------|
|         | Pred    | Avg   | Std  | SR    | Pred  | Avg   | Std  | SR    | Pred  | Avg   | Std  | SR    |
| Low(L)  | -0.17   | 0.00  | 7.97 | 0.00  | -0.88 | -0.33 | 6.59 | -0.17 | -0.72 | -0.50 | 7.04 | -0.25 |
| 2       | 0.12    | 0.19  | 6.53 | 0.10  | -0.26 | 0.27  | 5.83 | 0.16  | -0.13 | 0.16  | 6.14 | 0.09  |
| 3       | 0.31    | 0.40  | 5.72 | 0.24  | 0.06  | 0.35  | 5.41 | 0.22  | 0.16  | 0.36  | 5.52 | 0.22  |
| 4       | 0.45    | 0.52  | 5.32 | 0.34  | 0.31  | 0.54  | 5.16 | 0.36  | 0.39  | 0.52  | 5.21 | 0.35  |
| 5       | 0.58    | 0.63  | 4.96 | 0.44  | 0.54  | 0.66  | 5.01 | 0.46  | 0.59  | 0.63  | 4.94 | 0.44  |
| 6       | 0.70    | 0.63  | 4.71 | 0.46  | 0.75  | 0.70  | 4.97 | 0.49  | 0.77  | 0.71  | 4.83 | 0.51  |
| 7       | 0.82    | 0.66  | 4.64 | 0.49  | 0.96  | 0.82  | 4.71 | 0.60  | 0.96  | 0.76  | 4.80 | 0.55  |
| 8       | 0.96    | 0.75  | 4.70 | 0.56  | 1.21  | 0.85  | 5.12 | 0.57  | 1.17  | 0.95  | 4.84 | 0.68  |
| 9       | 1.15    | 1.04  | 4.95 | 0.73  | 1.53  | 1.02  | 5.32 | 0.66  | 1.46  | 1.09  | 5.14 | 0.74  |
| High(H) | 1.47    | 1.33  | 5.35 | 0.86  | 2.21  | 1.33  | 5.87 | 0.78  | 2.03  | 1.47  | 5.83 | 0.87  |
| H-L     | 1.64    | 1.32  | 5.66 | 0.81  | 3.09  | 1.66  | 4.69 | 1.22  | 2.75  | 1.97  | 4.61 | 1.48  |
| ENet+H  |         |       |      | GLM+H |       |       |      | RF    |       |       |      |       |
|         | Pred    | Avg   | Std  | SR    | Pred  | Avg   | Std  | SR    | Pred  | Avg   | Std  | SR    |
| Low(L)  | -0.05   | -0.23 | 6.51 | -0.12 | -0.51 | -0.35 | 6.81 | -0.18 | 0.27  | -0.43 | 7.03 | -0.21 |
| 2       | 0.25    | 0.42  | 5.72 | 0.26  | -0.03 | 0.32  | 5.71 | 0.20  | 0.44  | 0.23  | 5.58 | 0.15  |
| 3       | 0.42    | 0.53  | 5.14 | 0.36  | 0.25  | 0.54  | 5.34 | 0.35  | 0.52  | 0.50  | 5.19 | 0.33  |
| 4       | 0.56    | 0.60  | 4.82 | 0.43  | 0.45  | 0.59  | 5.12 | 0.40  | 0.59  | 0.58  | 5.04 | 0.40  |
| 5       | 0.69    | 0.69  | 4.80 | 0.50  | 0.63  | 0.65  | 4.98 | 0.45  | 0.66  | 0.58  | 4.97 | 0.41  |
| 6       | 0.82    | 0.73  | 4.89 | 0.52  | 0.79  | 0.68  | 4.96 | 0.48  | 0.72  | 0.65  | 5.04 | 0.45  |
| 7       | 0.96    | 0.83  | 4.74 | 0.61  | 0.95  | 0.70  | 4.91 | 0.49  | 0.78  | 0.65  | 4.99 | 0.45  |
| 8       | 1.11    | 0.77  | 5.31 | 0.50  | 1.12  | 0.75  | 4.95 | 0.53  | 0.85  | 0.85  | 5.02 | 0.58  |
| 9       | 1.30    | 0.78  | 5.74 | 0.47  | 1.34  | 0.95  | 5.30 | 0.62  | 0.92  | 1.08  | 5.34 | 0.70  |
| High(H) | 1.65    | 1.04  | 6.78 | 0.53  | 1.79  | 1.31  | 6.33 | 0.72  | 1.09  | 1.43  | 6.65 | 0.74  |
| H-L     | 1.70    | 1.27  | 4.90 | 0.90  | 2.30  | 1.65  | 4.44 | 1.29  | 0.81  | 1.86  | 5.25 | 1.22  |
| GBRT+H  |         |       |      | NN1   |       |       |      | NN2   |       |       |      |       |
|         | Pred    | Avg   | Std  | SR    | Pred  | Avg   | Std  | SR    | Pred  | Avg   | Std  | SR    |
| Low(L)  | -0.47   | -0.28 | 6.25 | -0.15 | -0.47 | -0.76 | 7.48 | -0.35 | -0.33 | -0.92 | 8.00 | -0.40 |
| 2       | -0.15   | 0.38  | 5.55 | 0.24  | 0.12  | 0.20  | 6.36 | 0.11  | 0.19  | 0.20  | 6.51 | 0.10  |
| 3       | 0.02    | 0.52  | 5.22 | 0.34  | 0.40  | 0.48  | 5.54 | 0.30  | 0.41  | 0.55  | 5.63 | 0.34  |
| 4       | 0.17    | 0.67  | 5.31 | 0.44  | 0.59  | 0.63  | 5.01 | 0.43  | 0.56  | 0.70  | 5.03 | 0.48  |
| 5       | 0.32    | 0.55  | 5.24 | 0.36  | 0.74  | 0.72  | 4.76 | 0.53  | 0.68  | 0.74  | 4.59 | 0.56  |
| 6       | 0.45    | 0.76  | 4.95 | 0.54  | 0.87  | 0.85  | 4.61 | 0.64  | 0.79  | 0.84  | 4.49 | 0.65  |
| 7       | 0.57    | 0.52  | 5.10 | 0.35  | 1.01  | 0.87  | 4.60 | 0.65  | 0.89  | 0.90  | 4.51 | 0.69  |
| 8       | 0.69    | 0.70  | 4.90 | 0.50  | 1.16  | 0.85  | 4.68 | 0.63  | 1.02  | 0.93  | 4.69 | 0.68  |
| 9       | 0.84    | 1.02  | 5.26 | 0.67  | 1.38  | 1.00  | 5.13 | 0.68  | 1.19  | 0.96  | 4.99 | 0.67  |
| High(H) | 1.10    | 1.30  | 6.25 | 0.72  | 1.91  | 1.29  | 6.25 | 0.72  | 1.68  | 1.26  | 6.22 | 0.70  |
| H-L     | 1.57    | 1.58  | 3.86 | 1.42  | 2.38  | 2.05  | 4.50 | 1.58  | 2.01  | 2.18  | 4.74 | 1.60  |
| NN3     |         |       |      | NN4   |       |       |      | NN5   |       |       |      |       |
|         | Pred    | Avg   | Std  | SR    | Pred  | Avg   | Std  | SR    | Pred  | Avg   | Std  | SR    |
| Low(L)  | -0.31   | -0.82 | 8.18 | -0.35 | -0.19 | -0.87 | 8.05 | -0.38 | -0.08 | -0.75 | 8.11 | -0.32 |
| 2       | 0.20    | 0.16  | 6.55 | 0.08  | 0.28  | 0.23  | 6.68 | 0.12  | 0.32  | 0.22  | 6.75 | 0.12  |
| 3       | 0.43    | 0.46  | 5.51 | 0.29  | 0.47  | 0.45  | 5.61 | 0.28  | 0.49  | 0.51  | 5.70 | 0.31  |
| 4       | 0.57    | 0.66  | 4.86 | 0.47  | 0.59  | 0.65  | 4.93 | 0.45  | 0.61  | 0.58  | 4.98 | 0.40  |
| 5       | 0.69    | 0.76  | 4.63 | 0.57  | 0.68  | 0.65  | 4.60 | 0.49  | 0.69  | 0.69  | 4.55 | 0.52  |
| 6       | 0.79    | 0.79  | 4.44 | 0.61  | 0.76  | 0.71  | 4.48 | 0.55  | 0.76  | 0.76  | 4.43 | 0.60  |
| 7       | 0.89    | 0.87  | 4.48 | 0.67  | 0.84  | 0.90  | 4.45 | 0.70  | 0.83  | 0.84  | 4.45 | 0.65  |
| 8       | 1.01    | 0.91  | 4.71 | 0.67  | 0.94  | 0.92  | 4.59 | 0.70  | 0.91  | 0.92  | 4.70 | 0.68  |
| 9       | 1.17    | 1.00  | 5.02 | 0.69  | 1.07  | 1.13  | 5.00 | 0.78  | 1.04  | 1.02  | 5.10 | 0.69  |
| High(H) | 1.64    | 1.37  | 6.34 | 0.75  | 1.52  | 1.39  | 6.37 | 0.75  | 1.48  | 1.36  | 6.34 | 0.74  |
| H-L     | 1.95    | 2.19  | 4.84 | 1.57  | 1.70  | 2.26  | 4.63 | 1.69  | 1.56  | 2.11  | 4.95 | 1.48  |

Note: In this table, we report the performance of prediction-sorted portfolios over the 30-year out-of-sample testing period. All but tiny stocks (excluding stocks below 20th percentile on NYSE cap weights) are sorted into deciles based on their predicted returns for the next month. Column “Pred”, “Avg”, “Std”, and “SR” provide the predicted monthly returns for each decile, the average realized monthly returns, their standard deviations, and Sharpe ratios, respectively. All portfolios are value weighted.

Table A.11: OLS Benchmark Models

| Model  | $R^2$ |         | Sharpe Ratio |              | Description                                        |
|--------|-------|---------|--------------|--------------|----------------------------------------------------|
|        | Stock | S&P 500 | Equal-weight | Value-weight |                                                    |
| OLS-3  | 0.16  | -0.22   | 0.83         | 0.61         | mom12m, size, bm                                   |
| OLS-7  | 0.18  | 0.24    | 1.12         | 0.74         | OLS-3 plus acc, roaq, agr, egr                     |
| OLS-15 | 0.19  | 0.68    | 1.15         | 0.86         | OLS-7 plus dy, mom36m, beta, retvol, turn, lev, sp |
| RF     | 0.33  | 1.37    | 1.48         | 0.98         |                                                    |
| NN3    | 0.40  | 1.80    | 2.36         | 1.20         |                                                    |

Note: In this table, we report the out-of-sample performance of three different OLS benchmark models recommended by Lewellen (2015) with either three, seven, or 15 predictors. We report predictive  $R^2$  for the stock-level panel and the S&P 500 index. We report long-short decile spread Sharpe ratios with equal-weight and value-weight formation. For comparison, we also report the performance the NN3 and random forest models.

Figure A.7: Cumulative Return of Machine Learning Portfolios (Equally Weighted)

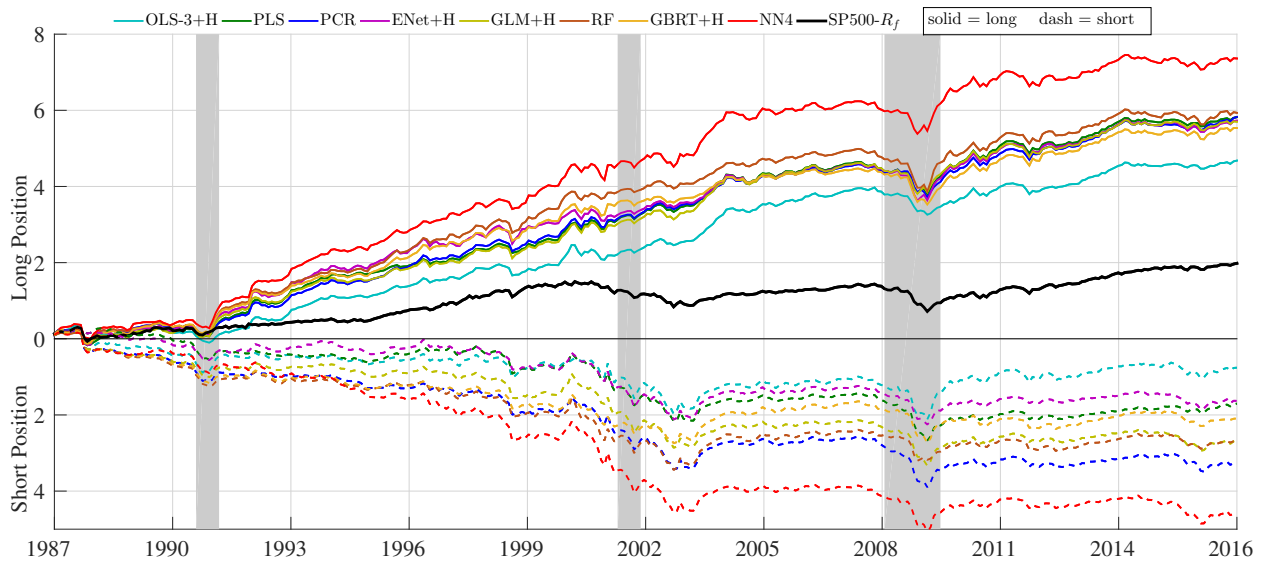

Note: Cumulative log returns of portfolios sorted on out-of-sample machine learning return forecasts. The solid and dash lines represent long (top decile) and short (bottom decile) positions, respectively. The shaded periods show NBER recession dates. All portfolios are equally weighted.

## References

- Bach, F. R. 2008. Consistency of the Group Lasso and Multiple Kernel Learning. *Journal of Machine Learning Research* 9:1179–1225. URL <http://dl.acm.org/citation.cfm?id=1390681.1390721>.
- Bai, J., and S. Ng. 2002. Determining the Number of Factors in Approximate Factor Models. *Econometrica* 70:191–221.
- Bai, J., and S. Ng. 2013. Principal components estimation and identification of static factors. *Journal of Econometrics* 176:18–29.

- Bai, Z. 1999. Methodologies in spectral analysis of large dimensional random matrices: A review. *Statistica Sinica* 9:611–677.
- Biau, G. 2012. Analysis of a Random Forests Model. *Journal of Machine Learning Research* 13:1063–1095.
- Bickel, P. J., Y. Ritov, and A. B. Tsybakov. 2009. Simultaneous analysis of Lasso and Dantzig selector. *Annals of Statistics* 37:1705–1732.
- Breiman, L., J. Friedman, C. J. Stone, and R. A. Olshen. 1984. *Classification and regression trees*. CRC press.
- Bühlmann, P., and T. Hothorn. 2007. Boosting Algorithms: Regularization, Prediction and Model Fitting. *Statistical Science* 22:477–505.
- Bühlmann, P., and B. Yu. 2003. Boosting With the L2 Loss. *Journal of the American Statistical Association* 98:324–339.
- Chen, T., and C. Guestrin. 2016. XGBoost: A Scalable Tree Boosting System. In *Proceedings of the 22Nd ACM SIGKDD International Conference on Knowledge Discovery and Data Mining, KDD '16*, pp. 785–794. New York, NY, USA: ACM. URL <http://doi.acm.org/10.1145/2939672.2939785>.
- Chizat, L., and F. Bach. 2018. On the Global Convergence of Gradient Descent for Overparameterized Models Using Optimal Transport. In *Proceedings of the 32Nd International Conference on Neural Information Processing Systems, NIPS'18*, pp. 3040–3050. USA: Curran Associates Inc. URL <http://dl.acm.org/citation.cfm?id=3327144.3327226>.
- Daubechies, I., M. Defrise, and C. De Mol. 2004. An iterative thresholding algorithm for linear inverse problems with a sparsity constraint. *Communications on Pure and Applied Mathematics* 57:1413–1457.
- Dimopoulos, Y., P. Bourret, and S. Lek. 1995. Use of some sensitivity criteria for choosing networks with good generalization ability. *Neural Processing Letters* 2:1–4.
- Eldan, R., and O. Shamir. 2016. The Power of Depth for Feedforward Neural Networks. In V. Feldman, A. Rakhlin, and O. Shamir (eds.), *29th Annual Conference on Learning Theory*, vol. 49 of *Proceedings of Machine Learning Research*, pp. 907–940. Columbia University, New York, New York, USA: PMLR. URL <http://proceedings.mlr.press/v49/eldan16.html>.
- Fan, J., Q. Li, and Y. Wang. 2017. Estimation of high dimensional mean regression in the absence of symmetry and light tail assumptions. *Journal of the Royal Statistical Society, B* 79:247–265.
- Fan, J., C. Ma, and Y. Zhong. 2019. A Selective Overview of Deep Learning. Tech. rep., Princeton University.

- Friedman, J., T. Hastie, H. Höfling, R. Tibshirani, et al. 2007. Pathwise coordinate optimization. *The Annals of Applied Statistics* 1:302–332.
- Friedman, J., T. Hastie, and R. Tibshirani. 2000. Additive logistic regression: a statistical view of boosting (With discussion and a rejoinder by the authors). *Annals of Statistics* 28:337–407. URL <https://doi.org/10.1214/aos/1016218223>.
- Friedman, J. H. 2001. Greedy function approximation: a gradient boosting machine. *Annals of statistics* pp. 1189–1232.
- Giglio, S. W., and D. Xiu. 2016. Asset Pricing with Omitted Factors. Tech. rep., University of Chicago.
- Goodfellow, I., Y. Bengio, and A. Courville. 2016. *Deep Learning*. MIT Press. <http://www.deeplearningbook.org>.
- Green, J., J. R. Hand, and X. F. Zhang. 2017. The characteristics that provide independent information about average us monthly stock returns. *The Review of Financial Studies* 30:4389–4436.
- Hastie, T., R. Tibshirani, and J. Friedman. 2009. *The Elements of Statistical Learning*. Springer.
- He, K., X. Zhang, S. Ren, and J. Sun. 2016. Deep Residual Learning for Image Recognition. In *The IEEE Conference on Computer Vision and Pattern Recognition (CVPR)*.
- Hornik, K., M. Stinchcombe, and H. White. 1989. Multilayer feedforward networks are universal approximators. *Neural networks* 2:359–366.
- Ioffe, S., and C. Szegedy. 2015. Batch Normalization: Accelerating Deep Network Training by Reducing Internal Covariate Shift. *International Conference on Machine Learning* pp. 448–456.
- Johnstone, I. M. 2001. On the distribution of the largest eigenvalue in principal components analysis. *Annals of Statistics* 29:295–327.
- Johnstone, I. M., and A. Y. Lu. 2009. On Consistency and Sparsity for Principal Components Analysis in High Dimensions. *Journal of the American Statistical Association* 104:682–693.
- Kelly, B., and S. Pruitt. 2013. Market expectations in the cross-section of present values. *The Journal of Finance* 68:1721–1756.
- Kelly, B., and S. Pruitt. 2015. The three-pass regression filter: A new approach to forecasting using many predictors. *Journal of Econometrics* 186:294–316.
- Kingma, D., and J. Ba. 2014. Adam: A method for stochastic optimization. *arXiv preprint arXiv:1412.6980* .
- Knight, K., and W. Fu. 2000. Asymptotics for lasso-type estimators. *Annals of Statistics* 28:1356–1378. URL <https://doi.org/10.1214/aos/1015957397>.

- Lewellen, J. 2015. The Cross-section of Expected Stock Returns. *Critical Finance Review* 4:1–44.
- Lin, H. W., M. Tegmark, and D. Rolnick. 2017. Why Does Deep and Cheap Learning Work So Well? *Journal of Statistical Physics* 168:1223–1247. URL <https://doi.org/10.1007/s10955-017-1836-5>.
- Lounici, K., M. Pontil, S. van de Geer, and A. B. Tsybakov. 2011. Oracle inequalities and optimal inference under group sparsity. *Annals of Statistics* 39:2164–2204. URL <https://doi.org/10.1214/11-AOS896>.
- Lugosi, G., and N. Vayatis. 2004. On the Bayes-risk consistency of regularized boosting methods. *Annals of Statistics* 32:30–55. URL <https://doi.org/10.1214/aos/1079120129>.
- Mei, S., T. Misiakiewicz, and A. Montanari. 2019. Mean-field theory of two-layers neural networks: dimension-free bounds and kernel limit. In *Conference on Learning Theory (COLT)*.
- Mei, S., A. Montanari, and P.-M. Nguyen. 2018. A mean field view of the landscape of two-layer neural networks. *Proceedings of the National Academy of Sciences* 115:E7665–E7671. URL <https://www.pnas.org/content/115/33/E7665>.
- Meinshausen, N., and B. Yu. 2009. Lasso-type recovery of sparse representations for high-dimensional data. *Annals of Statistics* 37:246–270.
- Mentch, L., and G. Hooker. 2016. Quantifying Uncertainty in Random Forests via Confidence Intervals and Hypothesis Tests. *Journal of Machine Learning Research* 17:1–41. URL <http://jmlr.org/papers/v17/14-168.html>.
- Mol, C. D., E. D. Vito, and L. Rosasco. 2009. Elastic-net regularization in learning theory. *Journal of Complexity* 25:201 – 230. URL <http://www.sciencedirect.com/science/article/pii/S0885064X0900003X>.
- Nesterov, Y. 1983. A method of solving a convex programming problem with convergence rate  $O(1/k^2)$ . *Soviet Mathematics Doklady* 27:372–376.
- Parikh, N., and S. Boyd. 2013. Proximal Algorithms. *Foundations and Trends in Optimization* 1:123–231.
- Paul, D. 2007. Asymptotics of Sample Eigenstructure for a Large Dimensional Spiked Covariance Model. *Statistical Sinica* 17:1617–1642.
- Polson, N. G., J. Scott, and B. T. Willard. 2015. Proximal Algorithms in Statistics and Machine Learning. *Statistical Science* 30:559–581.
- Ravikumar, P., J. Lafferty, H. Liu, and L. Wasserman. 2009. Sparse Additive Models. *Journal of the Royal Statistical Society. Series B (Statistical Methodology)* 71:1009–1030.

- Rolnick, D., and M. Tegmark. 2018. The power of deeper networks for expressing natural functions. In *ICLR*.
- Scornet, E., G. Biau, and J.-P. Vert. 2015. Consistency of random forests. *Annals of Statistics* 43:1716–1741. URL <https://doi.org/10.1214/15-AOS1321>.
- Stock, J. H., and M. W. Watson. 2002. Forecasting using Principal Components from a Large Number of Predictors. *Journal of American Statistical Association* 97:1167–1179.
- Tibshirani, R. 2011. Regression shrinkage and selection via the lasso: a retrospective. *Journal of the Royal Statistical Society: Series B (Statistical Methodology)* 73:273–282.
- Wager, S., and S. Athey. 2018. Estimation and Inference of Heterogeneous Treatment Effects using Random Forests. *Journal of the American Statistical Association* 113:1228–1242.
- Wager, S., T. Hastie, and B. Efron. 2014. Confidence Intervals for Random Forests: The Jackknife and the Infinitesimal Jackknife. *Journal of Machine Learning Research* 15:1625–1651. URL <http://jmlr.org/papers/v15/wager14a.html>.
- Wainwright, M. J. 2009. Sharp Thresholds for High-Dimensional and Noisy Sparsity Recovery Using  $l_1$ -Constrained Quadratic Programming (Lasso). *IEEE Transactions on Information Theory* 55:2183–2202.
- Wang, W., and J. Fan. 2017. Asymptotics of Empirical Eigenstructure for High Dimensional Spiked Covariance. *Annals of Statistics* 45:1342–1374.
- West, K. D. 2006. Forecast Evaluation. In G. Elliott, C. Granger, and A. Timmermann (eds.), *Handbook of Economic Forecasting*, vol. 1, pp. 99–134. Elsevier.
- Zhang, C.-H., and J. Huang. 2008. The sparsity and bias of the Lasso selection in high-dimensional linear regression. *Annals of Statistics* 36:1567–1594. URL <http://dx.doi.org/10.1214/07-AOS520>.
- Zhang, T., and B. Yu. 2005. Boosting with early stopping: Convergence and consistency. *Annals of Statistics* 33:1538–1579. URL <https://doi.org/10.1214/009053605000000255>.
- Zou, H., and T. Hastie. 2005. Regularization and Variable Selection via the Elastic Net. *Journal of the Royal Statistical Society. Series B (Statistical Methodology)* 67:301–320. URL <http://www.jstor.org/stable/3647580>.
- Zou, H., and H. H. Zhang. 2009. On the adaptive elastic-net with a diverging number of parameters. *Annals of Statistics* 37:1733–1751. URL <https://doi.org/10.1214/08-AOS625>.
