# Supplementary material for: Random Forest for Dynamic Risk Prediction or Recurrent Events: A Pseudo-Observation Approach
Source: arXiv:2312.00770 source file (2025-02-10)
Supplement: Supplementary file 3 [file rfre_po_supp.pdf]

# Supporting Information for “Random Forest for Dynamic Risk Prediction of Recurrent Events: A Pseudo-Observation Approach”

Abigail Loe<sup>1,\*</sup>, Susan Murray<sup>1,+</sup>, and Zhenke Wu<sup>1,+</sup>

<sup>1</sup>Department of Biostatistics, University of Michigan, Ann Arbor, MI 48109, USA; E-mail: \*agloe@umich.edu; +: co-senior authors

## A1 Tables and Figures

Table S1: XMT Model 1 parameter estimates, based on covariates selected by [Xia et al. \(2020\)](#), applied to censored longitudinal data with  $\tau = 180$ ,  $a = 30$ .

| Covariate                              | $e^{\hat{\beta}^\dagger}$ | 95% CI       | p             |
|----------------------------------------|---------------------------|--------------|---------------|
| Azithromycin (versus placebo)          | 1.43                      | (1.14, 1.79) | < <b>0.01</b> |
| Smoker at baseline (versus non-smoker) | 1.07                      | (0.80, 1.43) | 0.66          |
| FEV <sub>1</sub> in liters at baseline | 1.32                      | (1.05, 1.66) | <b>0.02</b>   |
| Male gender (versus female)            | 1.36                      | (1.07, 1.74) | <b>0.01</b>   |
| Age in decades                         | 1.14                      | (0.99, 1.32) | 0.07          |

<sup>†</sup>  $e^{\hat{\beta}}$  is the estimated odds ratio for being event-free during a 180-day follow-up period corresponding to a 1-unit increase in the (continuous) predictor, or the presence of a binary covariate, adjusted for other predictors.

FEV<sub>1</sub> is forced expiratory volume in one second, a clinical measure of lung function.

Correlation Matrix of Continuous Variables in Azithromycin Trial at Baseline

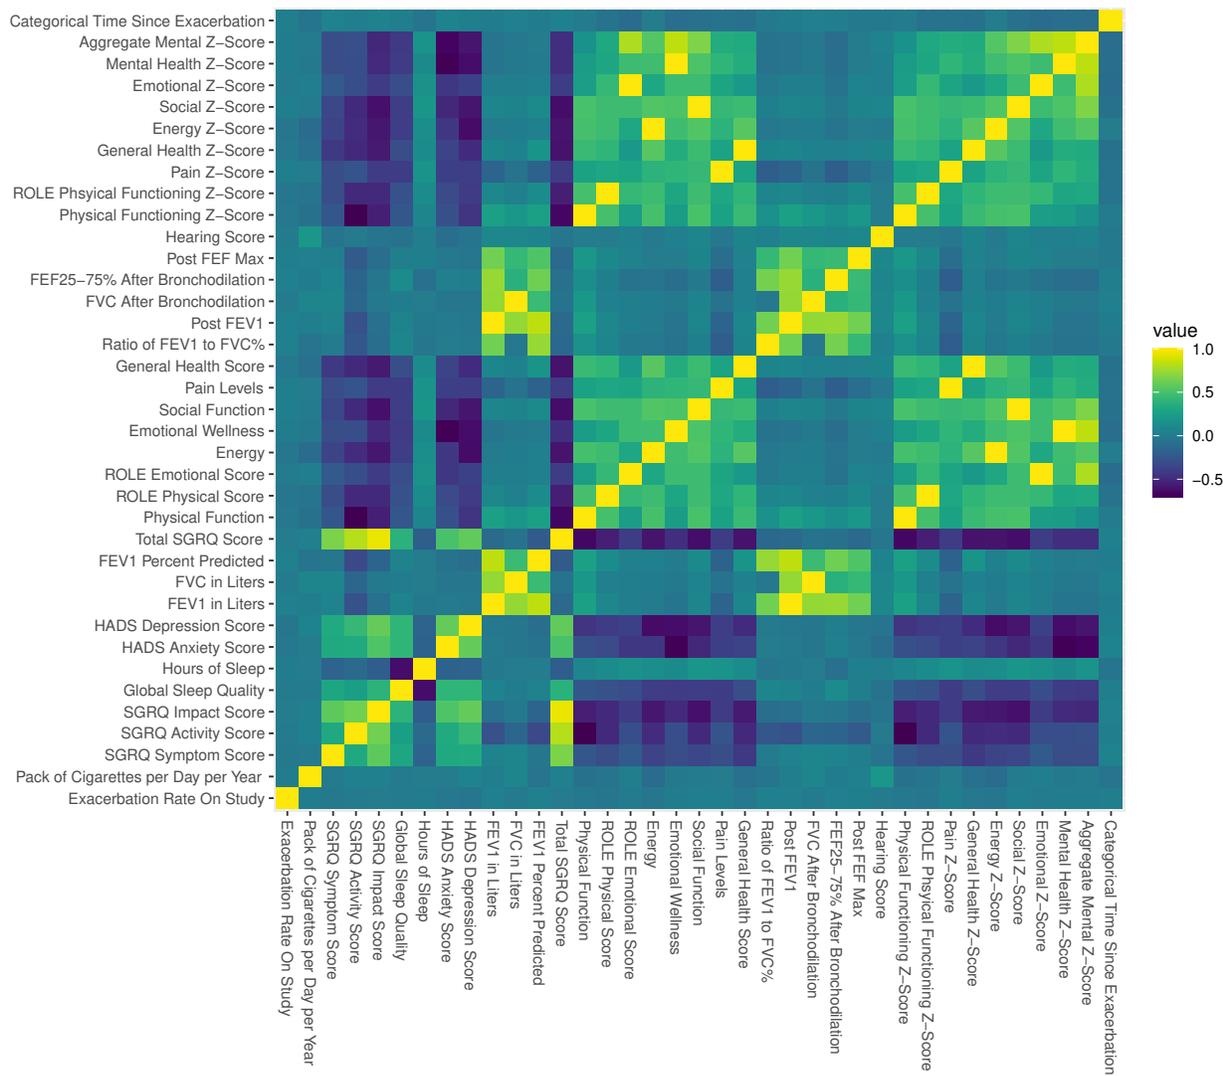

Figure S1: A correlation heat map of continuous and ordinal variables in the Azithromycin for the Prevention of COPD Cohort, measured at baseline. Variables derived from each other have instances of particularly high positive or negative correlation. These correlation patterns make random forest a more attractive modeling alternative compared to semi-parametric and parametric methods.

Table S2: Parameter Estimates from Model 2, or the model selected through Wald forward-selection on the first of  $m = 10$  imputed datasets. A very recent exacerbation, bronchitis, gender, treatment, the ratio of FEV to FVC %predicted, SGRQ symptoms, oxygen use, recent hospitalization, rate of exacerbations, and use of ICS medication remain significant across the  $m = 10$  imputed datasets. Exacerbation history indicators and rate of exacerbations are multiply imputed.

| Covariate                                                                            | $e^{\hat{\beta}}$ † | 95% CI       | p             |
|--------------------------------------------------------------------------------------|---------------------|--------------|---------------|
| Exacerbation in the 0-30 days prior to time $t$<br>(versus more than 30 days)        | 2.18                | (1.91, 2.48) | < <b>0.01</b> |
| Bronchiectasis diagnosis at time $t$ (versus no diagnosis)                           | 0.60                | (0.44, 0.81) | < <b>0.01</b> |
| Male gender (versus female gender)                                                   | 1.94                | (1.43, 2.64) | < <b>0.01</b> |
| Azithromycin (versus placebo)                                                        | 1.62                | (1.20, 2.18) | < <b>0.01</b> |
| Non-selective beta-blocker use at time $t$<br>(versus selective and no beta-blocker) | 0.14                | (0.00, 5.71) | 0.30          |
| Mixed beta-blocker use at time $t$<br>(versus selective and no beta-blocker)         | 2.54                | (0.98, 6.59) | <b>0.05</b>   |
| FEV <sub>1</sub> /FVC % predicted at time $t$                                        | 1.01                | (1.00, 1.02) | <b>0.03</b>   |
| SGRQ symptoms at time $t$                                                            | 0.99                | (0.99, 1.00) | <b>0.03</b>   |
| Supplemental oxygen use at time $t$<br>(versus no supplemental oxygen)               | 0.74                | (0.55, 0.99) | <b>0.04</b>   |
| Hospitalization in the year before study time<br>(versus not hospitalized)           | 0.60                | (0.45, 0.80) | < <b>0.01</b> |
| Rate of exacerbation prior to time $t$                                               | 1.25                | (1.05, 1.50) | <b>0.01</b>   |
| Corticosteroid and long-acting muscarinic antagonist use at time $t$<br>(versus not) | 0.72                | (0.55, 0.95) | <b>0.02</b>   |
| Corticosteroid and long-acting beta-agonist use at time $t$<br>(versus not)          | 1.30                | (1.03, 1.63) | <b>0.03</b>   |

†:  $e^{\hat{\beta}}$  is the estimated odds ratio for being event-free during a 180-day follow-up period corresponding to a 1-unit increase in the (continuous) predictor, or the presence of a binary covariate, adjusted for other predictors.

FEV<sub>1</sub> is forced expiratory volume in one second and FVC is forced vital capacity, clinical measures of lung function.

SGRQ is the Saint George's Respiratory Questionnaire, a patient reported outcome measuring quality of life.

Table S3: P-values from the RFRE.PO permutation test applied to the out-of-bag-samples combined across  $m = 10$  multiply imputed datasets. Included predictors had a statistically significant permutation test z-score for at least one of the multiply imputed training datasets. Additional predictors that did not achieve statistical significance via the permutation test, but were used in the RFRE.PO algorithm in some form, are not shown.

| Covariate                                                                          | p             |
|------------------------------------------------------------------------------------|---------------|
| Exacerbation in the 0-30 days prior to time $t$                                    | <b>0.04</b>   |
| Exacerbation in the 31-92 days prior to time $t$                                   | 0.06          |
| Exacerbation in the 366+ days (or none) prior to time $t$                          | <b>0.01</b>   |
| Categorical time since most recent exacerbation prior to time $t$ , or $H_{p1}(t)$ | 0.79          |
| Rate of Exacerbation                                                               | 0.61          |
| Had a severe exacerbation on study time prior to time $t$                          | 0.05          |
| General health score at time $t$                                                   | 0.90          |
| Standardized general health z-score at time $t$                                    | < <b>0.01</b> |
| Male gender                                                                        | < <b>0.01</b> |
| Anti-coagulant use at time $t$                                                     | <b>0.01</b>   |
| Pain score at time $t$                                                             | < <b>0.01</b> |
| Standardized pain z-score at time $t$                                              | 0.26          |
| FEV <sub>1</sub> in liters at time $t$                                             | <b>0.01</b>   |
| Treatment group                                                                    | 0.42          |
| SGRQ symptoms at time $t$                                                          | < <b>0.01</b> |
| Long-acting beta-agonist use at time $t$                                           | 0.90          |
| Long-acting muscarinic antagonist use at time $t$                                  | <b>0.02</b>   |
| Inhaled corticosteroids use in the year before study time                          | 0.07          |
| Hospitalization in the year before study time                                      | 0.38          |
| Phlegm at time $t$                                                                 | 0.51          |
| Baseline smoking                                                                   | 0.05          |
| Leukocytosis at time $t$                                                           | 0.05          |
| Oxygen use at time $t$                                                             | 0.07          |
| Bronchiectasis diagnosis at time $t$                                               | 0.50          |
| FEV <sub>1</sub> /FVC % Predicted at time $t$                                      | 0.40          |
| Saw a mental health provider for depression or anxiety at time $t$                 | 0.53          |
| Anxiety HADS score at time $t$                                                     | 0.21          |

FEV<sub>1</sub> is forced expiratory volume in one second and FVC is forced vital capacity, clinical measures of lung function.

SGRQ is the Saint George's Respiratory Questionnaire, a patient reported outcome measuring quality of life.

HADS Anxiety score Hospital Anxiety and Depression Scale is a clinical measure of mental well-being.

## References

Xia, M., Murray, S., and Tayob, N. (2020). Regression analysis of recurrent-event-free time from multiple follow-up windows. *Statistics in Medicine*, 39:1–15.
